# Supplementary material for: Convex block-sparse linear regression with expanders -- provably
Source: arXiv:1603.06313 source file (2016-04-03)
Supplement: Supplementary file 1 [file appendix.tex]

\section{Appendix}

\subsection{Proof of Theorem \ref{thm:mdlexpander_lg}}

We use a standard probabilistic argument to show that such matrices exist with non-negligible probability \cite{indyk2013model}. Let $\model_t^l$ denote a collection of $t$ blocks: assuming that each $\mathcal{G}_j \in \model_t^l$ has cardinality $|\mathcal{G}_j| = g$ for $g \ll \dim$, we have $|\model_t^l| = t \cdot g$. 

Two useful inequalities are given next: for $\dim \in \mathbb{Z}_{+}, ~v \in [0, 1]$ such that $v\dim \in \mathbb{Z}_{+}$, we have \cite{cheney1966introduction}:
\begin{align}{\label{eq:app_00}}
{\dim \choose \dim v} \leq \frac{5e^{\dim\cdot \mathcal{H}(v)}}{4\sqrt{2\pi v(1-v) \dim}},
\end{align} where $\mathcal{H}(v) = -v\log v - (1-v) \log(1-v)$. Also, \cite{bah2014bounds}:
\begin{align}{\label{eq:app_03}}
\mathcal{H}(x) < -x\log x + x.
\end{align}

Assume a binary expander graph $\left(\dim, \numsam, \EE \right)$. For given set $\mathcal{S}$ of size $|\mathcal{S}| = s, ~\mathcal{S} \in\dim$, we define the event:
\begin{align}
\Omega_{\mathcal{S}} := |\left\{j \in [\numsam] ~:~\exists i \in \mathcal{S}, ~(i,j) \in \EE \right\}| \geq (1 - \epsilon)ds \label{eq:app_07}
\end{align} For our analysis, we use the following lemmata; the proof is provided in \cite{buhrman2002bitvectors}:
\begin{lemma}{\label{lemma:app_01}}
There exist constants $\tilde{C} > 1$ and $\mu > 0$ such that, whenever $\numsam \geq \tilde{C}ds/\epsilon$, for any $\mathcal{S} \subseteq [\dim]$ with $|\mathcal{S}| = s,$ one has:
\begin{align*}
\mathbb{P}\left\{ \Omega_\mathcal{S}^c\right\} \leq \left(\mu \cdot \frac{\epsilon \numsam}{ds}\right)^{-\epsilon d s}
\end{align*}
\end{lemma} In our block sparse context, $\mathcal{S}$ is $\model_t^l$, for some $l$, $\epsilon = \epsilon_{\model_\sparsity}$ and $\mathbb{P}\left\{ \Omega_{\model_t^l}^c\right\} \leq \left(\mu \cdot \frac{\epsilon_{\model_\sparsity} \cdot \numsam}{d \cdot |\model_t^l|}\right)^{-\epsilon_{\model_\sparsity} \cdot d \cdot |\model_t^l|} $.

\begin{lemma}[\cite{bah2014model}]{\label{lemma:app_04}}
Given group size $k$, for all $t \in [\sparsity]$ and $M$ groups in our model, we have ${M \choose t}$
number of distinct $t$-block-sparse sets $\model_t^l, ~l \in \left\{1, \dots, {M \choose t}\right\}$, each one with cardinality $|\model_t^l| = t g$.
\end{lemma}

We construct $\Ph \in \left\{0, 1\right\}^{\numsam \times \dim}$ as follows: Given properly selected $\numsam$ and $d$ quantities, for each left-node (index) in $[\dim]$ independently, we select $d$ right-nodes in $[\numsam]$ to connect, uniformly at random.
%We are interested in bounding the probability of existence of expander graphs, under the assumption of block sparse signals. 
Using this construction and Lemma \ref{lemma:app_01}, we desire to bound away from zero the probability that \emph{every} $t$-block sparse set $\model_t^l$, $t \in [k]$, is ``expanded'' properly using $\Ph$. This translates in bounding the probability:% one can bound the probability \textcolor{magenta}{\textbf{What does this bound mean?}}, as follows:
\begin{align*}
\mathbb{P}&\left\{ \cap_{t = 1}^\sparsity \cap_{l = 1}^{{M \choose t}} \Omega_{\model_t^l}\right\} \stackrel{(i)}{\geq} 1 - \sum_{t = 1}^\sparsity \sum_{l = 1}^{{M \choose t}} \mathbb{P}\left\{ \Omega_{\model_t^l}^c\right\} \\
&\stackrel{(ii)}{\geq} 1 - \sum_{t = 1}^\sparsity \sum_{l = 1}^{{M \choose t}} \left(\mu \cdot \frac{\epsilon_{\model_\sparsity} \cdot \numsam}{  d \cdot |\model_t^l|}\right)^{-\epsilon_{\model_\sparsity} \cdot |\model_t^l| \cdot d } \\
&= 1 - \sum_{t = 1}^\sparsity \sum_{l = 1}^{{M \choose t}} e^{-\epsilon_{\model_\sparsity} \cdot |\model_t^l| \cdot d \cdot \log\left(\mu \cdot \frac{\epsilon_{\model_\sparsity} \cdot \numsam}{  d \cdot |\model_t^l|}\right)} \\
& \stackrel{(iii)}{=} 1 - \sum_{t = 1}^\sparsity \sum_{l = 1}^{{M \choose t}} e^{- \epsilon_{\model_\sparsity} \cdot d\cdot t \cdot g \cdot \log \left(\mu \cdot \frac{\epsilon_{\model_\sparsity} \cdot \numsam}{  d \cdot t \cdot g}\right)} \\
%& \stackrel{(iv)}{\geq} 1 - \sum_{t = 1}^\sparsity \sum_{l = 1}^{{M \choose t}} e^{- \epsilon_{\model_\sparsity} \cdot d \cdot t \cdot \log \left(\mu \cdot \frac{\epsilon_{\model_\sparsity} \cdot \numsam}{  d \cdot t \cdot g_{\max}}\right)} \nonumber \\ 
&= 1 - \sum_{t = 1}^\sparsity {M \choose t} e^{-\epsilon_{\model_\sparsity} \cdot d \cdot t \cdot g \cdot \log \left(\mu \cdot \frac{\epsilon_{\model_\sparsity} \cdot \numsam}{  d \cdot t \cdot g}\right)} \nonumber \\ 
&\stackrel{(iv)}{\geq}  1 - \sum_{t = 1}^\sparsity \frac{5\sqrt{M}}{4\sqrt{2\pi t \left(M - t\right)}} \\ &\cdot e^{M \cdot \mathcal{H}(\frac{t}{M}) - \epsilon_{\model_\sparsity} \cdot d \cdot t \cdot g \cdot \log \left(\mu \cdot \frac{\epsilon_{\model_\sparsity} \cdot \numsam}{  d \cdot t \cdot g}\right)} \\
\end{align*} where $(i)$ is due to De Morgan's Law and the Union Bound, $(ii)$ is by using Lemma \ref{lemma:app_01}, $(iii)$ is due to the fact that $|\model_t^l| = t g, \forall i,$ and, $(iv)$ is due to \eqref{eq:app_00}. To proceed, we use the following Lemma.%; the proof is provided in the supplementary material.

\begin{lemma}{\label{lemma:app_03}}
Let $M, \sparsity \in \mathbb{Z}_{+}, ~M > \sparsity \geq 2$ and $t \in \mathbb{Z}_{+}$ such that $t \in [\sparsity]$. Define the function:
\begin{align*}
g(t) = \frac{5\sqrt{M}}{4\sqrt{2\pi t (M - t)}}.
\end{align*} Then, $0 < g(t) < 1, ~\forall t \in [\sparsity]$.
\end{lemma}
\begin{proof}
We observe:
\begin{align}
\frac{\partial g(t)}{\partial t} &= -\frac{5\sqrt{M}}{8\sqrt{2\pi}} \frac{M - 2t}{\sqrt[3]{t^2(M - t)^2}}, \nonumber %\label{eq:app_08}
\end{align} and 
\begin{align*}
\frac{\partial^2 g(t)}{\partial t^2} = \frac{c}{2} \left( \frac{3}{2} \frac{(M - 2t)^2}{\sqrt[5]{t^2 (M-t)^2}} + \frac{2}{\sqrt[3]{t^2(M - t)^2}} \right) > 0, 
\end{align*} $\forall t \in [\sparsity], $ i.e., $g(t)$ is convex function with minimum at $t^{\star} = \frac{M}{2}$ in \eqref{eq:app_08}. 
Thus, $f$ is a monotonically decreasing function in the domain $t \in [\sparsity]$. Computing the value of $g$ at points $t = 1,~t = \sparsity$, we observe:
\begin{align*}
g(t)\Big|_{t = 1} &= \frac{5}{4\sqrt{2\pi}} \left(1 + \frac{1}{M - 1}\right)^{1/2} \nonumber \\ &\stackrel{(i)}{<} \frac{5}{4\sqrt{2\pi}} \left(1 + 2 \frac{1}{M - 1}\right) \\ &\stackrel{(ii)}{<} 1,
\end{align*} where $(i)$ is due to the Taylor expansion upper bound of the term $(1 + 1/(m-1))^{1/2}$ and, $(ii)$ is due to the fact that $M \geq 2$, and
\begin{align*}
g(t)\Big|_{t = \sparsity} = \frac{5}{4\sqrt{2\pi}} \frac{1}{\sqrt{\sparsity\left( 1 - \frac{\sparsity}{M}\right)}},
\end{align*} since $\sparsity \geq 2$ and $D \geq 2$. Thus, $g(t) < 1, ~\forall t \in [\sparsity]$.	

\end{proof}

Thus, we may safely deduce that:
\begin{align}
\mathbb{P}&\left\{ \cap_{t = 1}^\sparsity \cap_{l = 1}^{{M \choose t}} \Omega_{\model_t^l}\right\} \nonumber \\
&\geq 1 - \sum_{t = 1}^\sparsity e^{M \cdot \mathcal{H}(\frac{t}{M}) - \epsilon_{\model_\sparsity} \cdot d \cdot t \cdot g \cdot \log \left(\mu \cdot \frac{\epsilon_{\model_\sparsity} \cdot \numsam}{  d \cdot t \cdot g}\right)} \nonumber \\ 
&= 1 - \sum_{t = 1}^\sparsity e^{\psi(d, t, \epsilon_{\model_\sparsity})} \label{eq:app_08}
\end{align} In the last equation, we define $\psi(d, t, \epsilon_{\model_\sparsity}) := M \cdot \mathcal{H}\left(\frac{t}{M}\right) - \epsilon_{\model_\sparsity} \cdot d \cdot t \cdot g \cdot \log \left(\mu \cdot \frac{\epsilon_{\model_\sparsity} \cdot \numsam}{  d \cdot t \cdot g}\right)$. First, we require to find the conditions that lead to $\psi(d, t, \epsilon_{\model_\sparsity}) \leq 0$, such that the above probability is valid. In particular, we have:
\begin{footnotesize}
\begin{align*}
&\psi(d, t, \epsilon_{\model_\sparsity}) \nonumber \\ &= M \cdot \mathcal{H}\left(\frac{t}{M}\right) - \epsilon_{\model_\sparsity} \cdot d \cdot t \cdot g \cdot \log \left(\mu \cdot \frac{\epsilon_{\model_\sparsity} \cdot \numsam}{  d \cdot t \cdot g}\right) \\
							  &\stackrel{(i)}{=} M\cdot \mathcal{H}\left(\frac{t}{M}\right) - \epsilon_{\model_\sparsity} \cdot d \cdot t \cdot g \cdot \log \left(C_2 \cdot \mu\right) \\
							  &\stackrel{(ii)}{<} M\cdot \left(-\frac{t}{M} \log\frac{t}{M}+ \frac{t}{M}\right) - \epsilon_{\model_\sparsity} \cdot d \cdot t \cdot g \cdot \log \left(C_2 \cdot \mu\right) \\
							  &\stackrel{}{=} -t\log(t) + t\cdot \left(\log M + 1\right) - \epsilon_{\model_\sparsity} \cdot d \cdot t \cdot g \cdot \log \left(C_2\cdot \mu\right) \\
							  &\stackrel{}{<} t\log \left(M e\right) - \epsilon_{\model_\sparsity} \cdot d \cdot t \cdot g \cdot \log \left(C_2 \cdot \mu\right) 
\end{align*}
\end{footnotesize} where $(i)$ is due to assuming that $\numsam = C_2 \cdot \frac{  d \cdot t \cdot g}{\epsilon_{\model_\sparsity}} = \mathcal{O}\left(\frac{d\cdot t \cdot g}{\epsilon_{\model_\sparsity}}\right)$ for some constant $C_2 > 0$, $(ii)$ is due to \eqref{eq:app_03}. The right hand side to be $< 0$ we require:
\begin{align}
\psi(d, t, \epsilon_{\model_\sparsity}) < 0 \Leftrightarrow d \geq C_3 \cdot \frac{\log M}{g \cdot \epsilon_{\model_\sparsity}}, \nonumber
\end{align} for a constant $C_3 > 0$. %i.e., $d = \mathcal{O}\left(\frac{\log M}{\epsilon_{\model_\sparsity}}\right)$. 
To conclude, let us find the conditions such that: $\mathbb{P}\left\{ \cap_{t = 1}^\sparsity \cap_{l = 1}^{{M \choose t}} \Omega_{\model_t^l}\right\} \geq 1 - \eta,~ \eta \in (0,1)$; this holds if in \eqref{eq:app_08} we have:
\begin{align*}
1 - \sum_{t = 1}^\sparsity e^{\psi(d, t, \epsilon_{\model_\sparsity})} \geq 1 - \eta 
\end{align*} which holds if 
\begin{align*}
\sparsity \cdot e^{\psi(d, 1, \epsilon_{\model_\sparsity})} \leq \eta.
\end{align*} Based on the bound of the function $\psi$ above, this is satisfied if:
\begin{align*}
\sparsity \cdot e^{\log(M e) - \epsilon_{\model_\sparsity} \cdot d \cdot g \cdot \log(C_2 \cdot \mu)} \leq \eta
\end{align*} This leads to the following requirement:
\begin{small}\begin{align*}
d \geq C_4 \cdot \frac{\log \sfrac{(\sparsity M)}{\eta}}{g \cdot \epsilon_{\model_\sparsity}} \left(\geq C_3 \cdot \frac{\log M}{g \cdot \epsilon_{\model_\sparsity}}\right) 
\end{align*}\end{small} for a properly selected constant $C_4 > 0$.
%require we obtain
%\begin{align*}
%\mathbb{P}\left\{ \cap_{t = 1}^\sparsity \cap_{l = 1}^{{M \choose t}} \Omega_{\model_t}\right\} &\stackrel{(v)}{\geq} 1 - \sum_{t = 1}^\sparsity e^{-\beta t} \\ &\geq 1 - \sum_{t = 1}^\infty e^{-\beta t} \\ &= \frac{1}{e^\beta -1} > 0.
%\end{align*} where in $(v)$ $\beta := \epsilon_{\model_\sparsity} \cdot d \cdot \log (C_1 \cdot \mu) - \log (Me) > 0$. 
\textit{I.e.}, there exists a probabilistic construction for model-based expander matrices where, for any $d \geq C_4 \cdot \frac{ \log \sfrac{(\sparsity M)}{\eta}}{g \cdot \epsilon_{\model_\sparsity}}$, $\numsam = \mathcal{O}\left(\frac{d \cdot \sparsity \cdot g}{\epsilon_{\model_\sparsity}}\right)$ measurements are sufficient for $\Ph$ to satisfy the model-RIP-1 \eqref{eqn:mrip2} with non-negligible probability. This completes the proof.

%\subsection{Proof of Lemma \ref{lemma:app_03}}

\input{comparison}

\section{More experimental results}
Here, we report further results on the 2D image recovery problem. We remind that, for the purpose of this experiment, we set up an upper wall time of $10^4$ seconds (\textit{i.e.}, $~2.8$ hours) to process $100$ frames for each solver. This translates into $100$ seconds per frame.

\subsection{Varying group size $g$}
For this case, we focus on a single frame. Due to its higher number of non-zeros, we have selected the frame shown in Figure \ref{fig:003}. For this case, we consider a roughly sufficient number of measurements is acquired where $\numsam = \lceil 0.3 \cdot \dim \rceil$. By varying the group size $g$, we obtain the results in Figure \ref{fig:003}. 

\subsection{Varying number of measurements}
Here, let $g = 4$ as this group selection performs better, as shown in the previous subection. Here, we consider $\numsam$ take values from $\numsam \in \left\lceil \left\{ 0.25, 0.3, 0.35, 0.4 \right\} \cdot \dim \right \rceil$. The results, are shown in Figure \ref{fig:004}.

\begin{figure*}[t]
\centering
	\begin{minipage}{0.15\linewidth}
	\centering \small{Original}
	\end{minipage}
	\begin{minipage}{0.15\linewidth}
	\centering \small{$\ell_1$ + Exp.}
	\end{minipage}
	\begin{minipage}{0.15\linewidth}
	\centering \small{$\ell_1$ + Gaus.}
	\end{minipage}
	\begin{minipage}{0.15\linewidth}
	\centering \small{$\ell_{2,1}$ + Exp.}
	\end{minipage}
	\begin{minipage}{0.15\linewidth}
	\centering \small{$\ell_{2,1}$ + Gaus.}
	\end{minipage}\\
	\includegraphics[width = 0.18\linewidth]{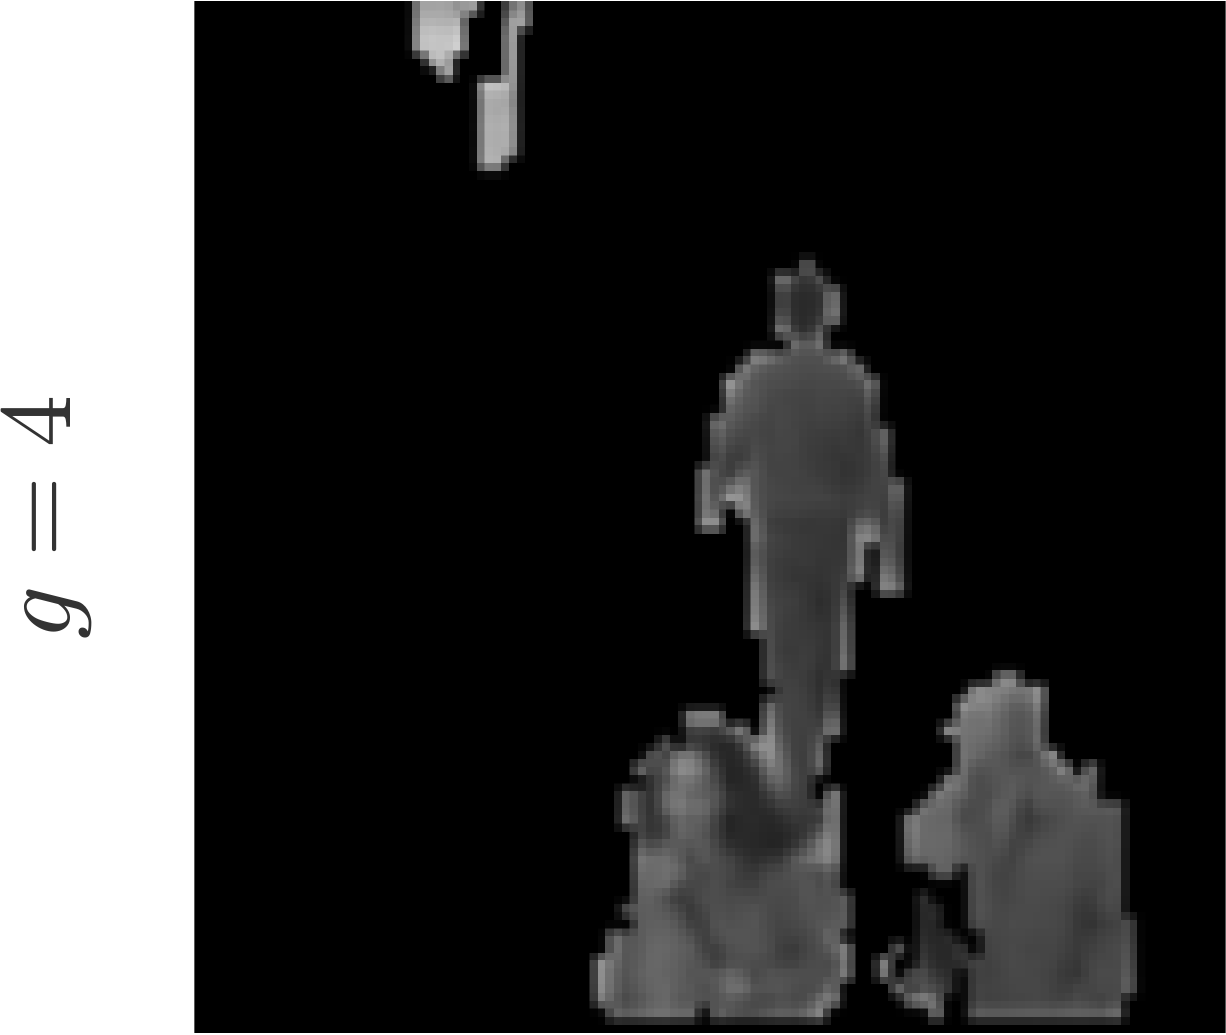}
	\includegraphics[width = 0.15\linewidth]{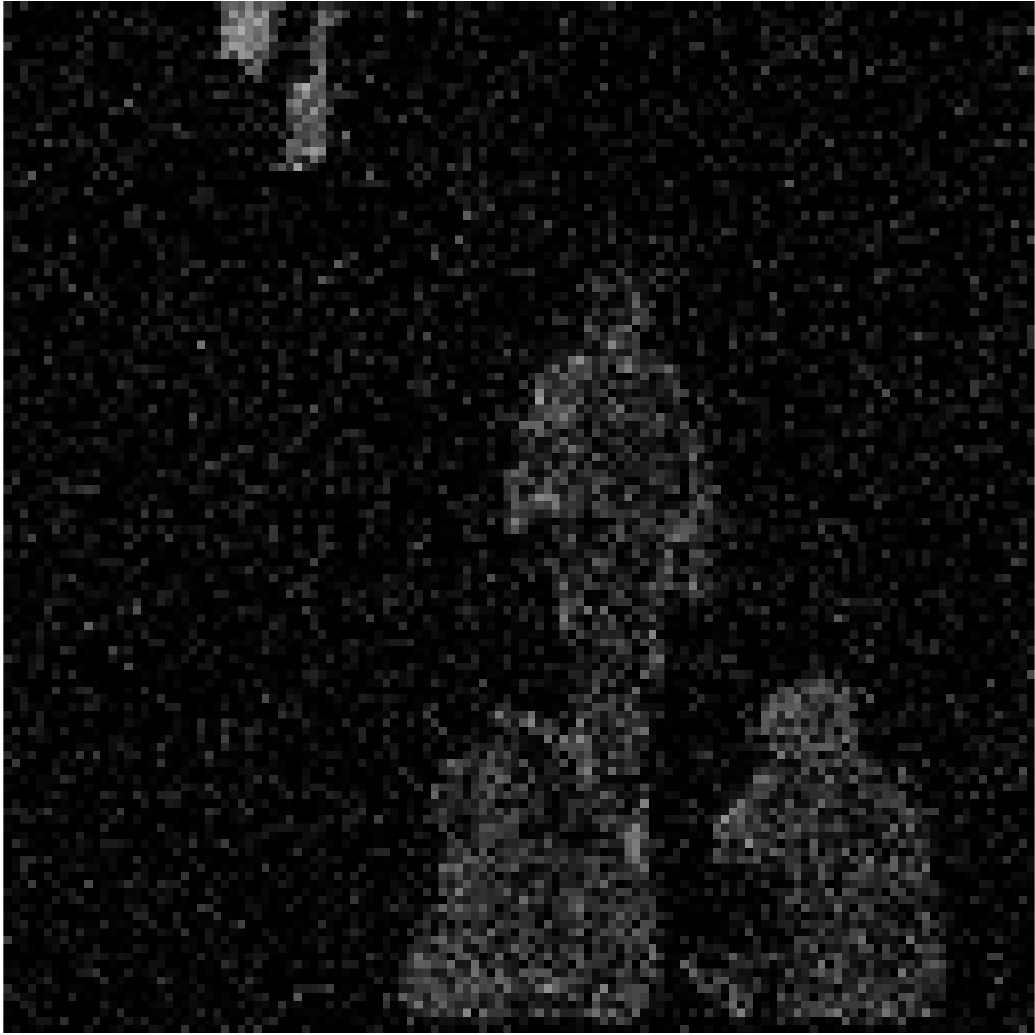}
	\includegraphics[width = 0.15\linewidth]{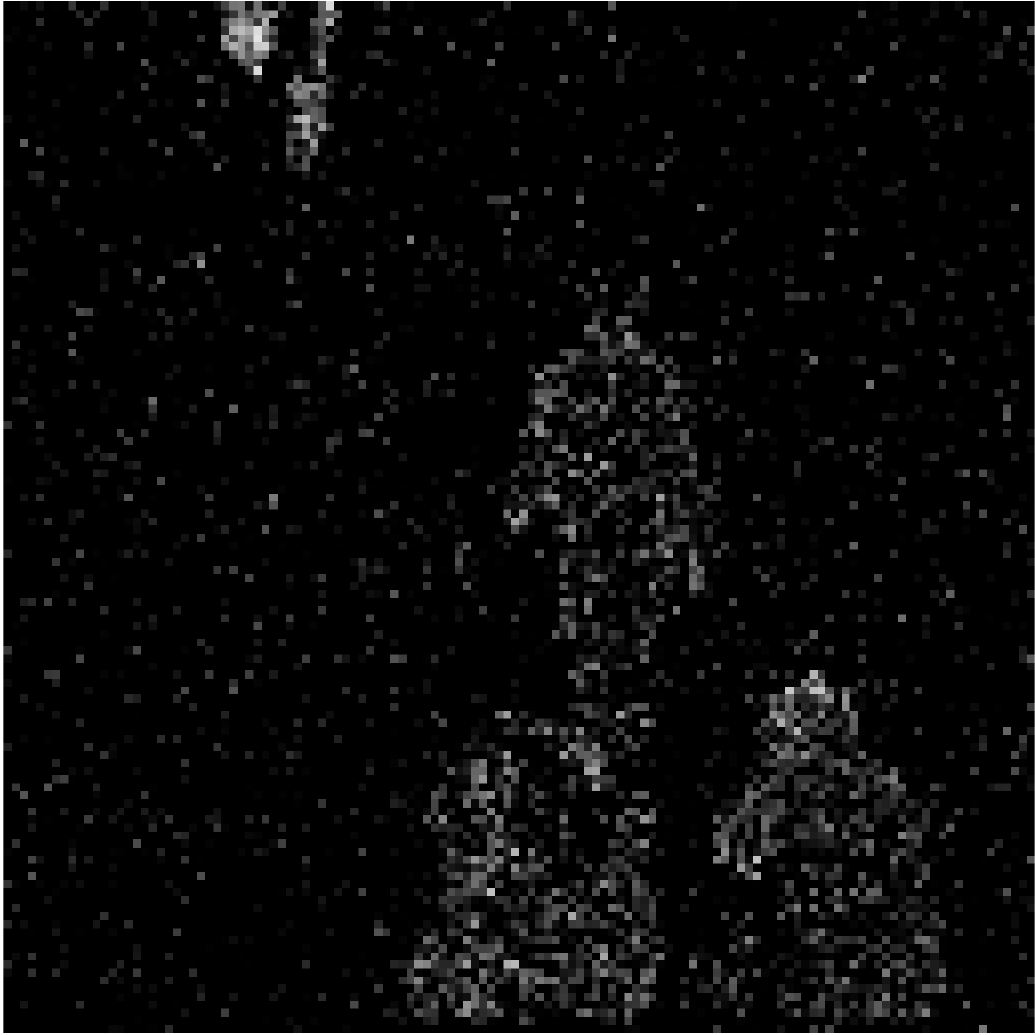}
	\includegraphics[width = 0.15\linewidth]{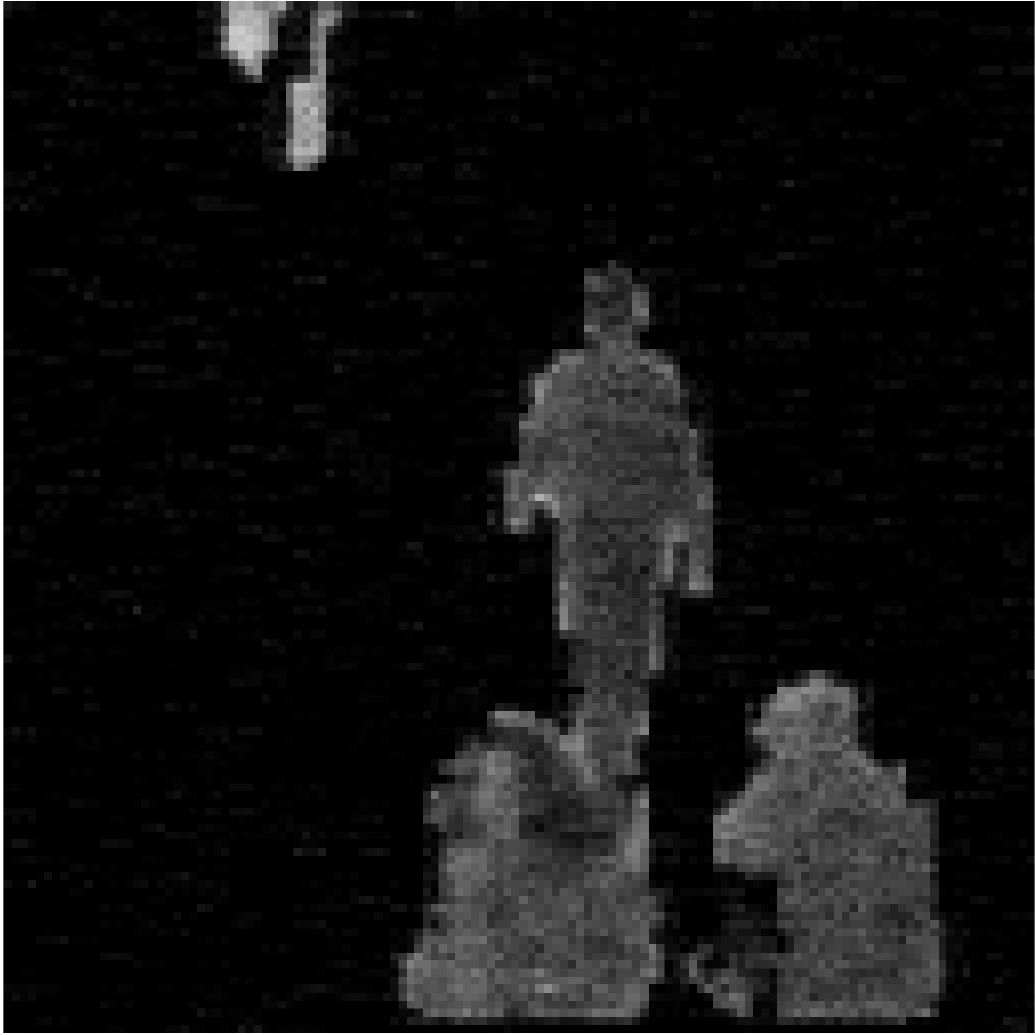}
	\includegraphics[width = 0.15\linewidth]{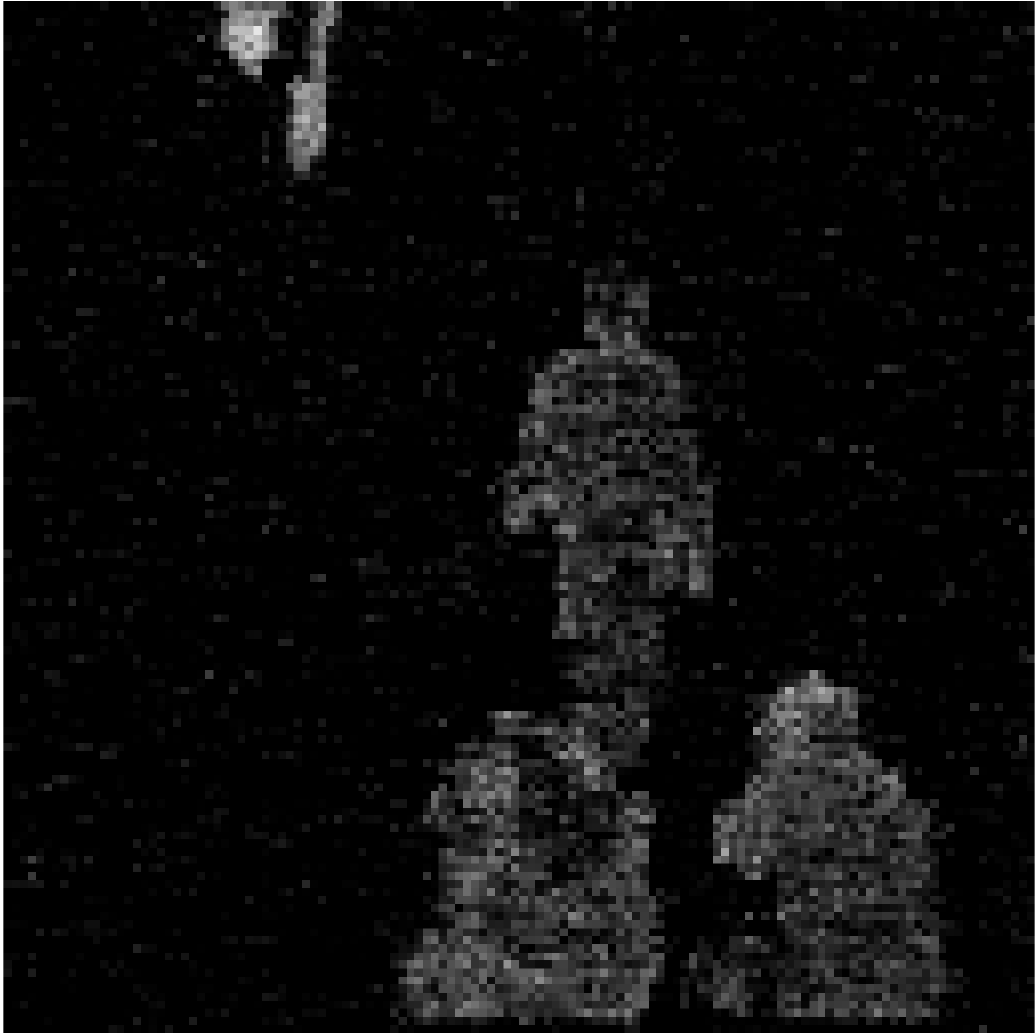} \vspace{-2mm} \\	
	\begin{minipage}{0.15\linewidth}
	\centering  \small{$\phantom{a}$}
	\end{minipage}	
	\begin{minipage}{0.15\linewidth}
	\centering  \small{$20.6 ~\rm{dB}$}
	\end{minipage}
	\begin{minipage}{0.15\linewidth}
	\centering \small{$18.5 ~\rm{dB}$}
	\end{minipage}
	\begin{minipage}{0.15\linewidth}
	\centering \small{$31.5 ~\rm{dB}$}
	\end{minipage}
	\begin{minipage}{0.15\linewidth}
	\centering \small{$24.8 ~\rm{dB}$}
	\end{minipage}\\
	\includegraphics[width = 0.18\linewidth]{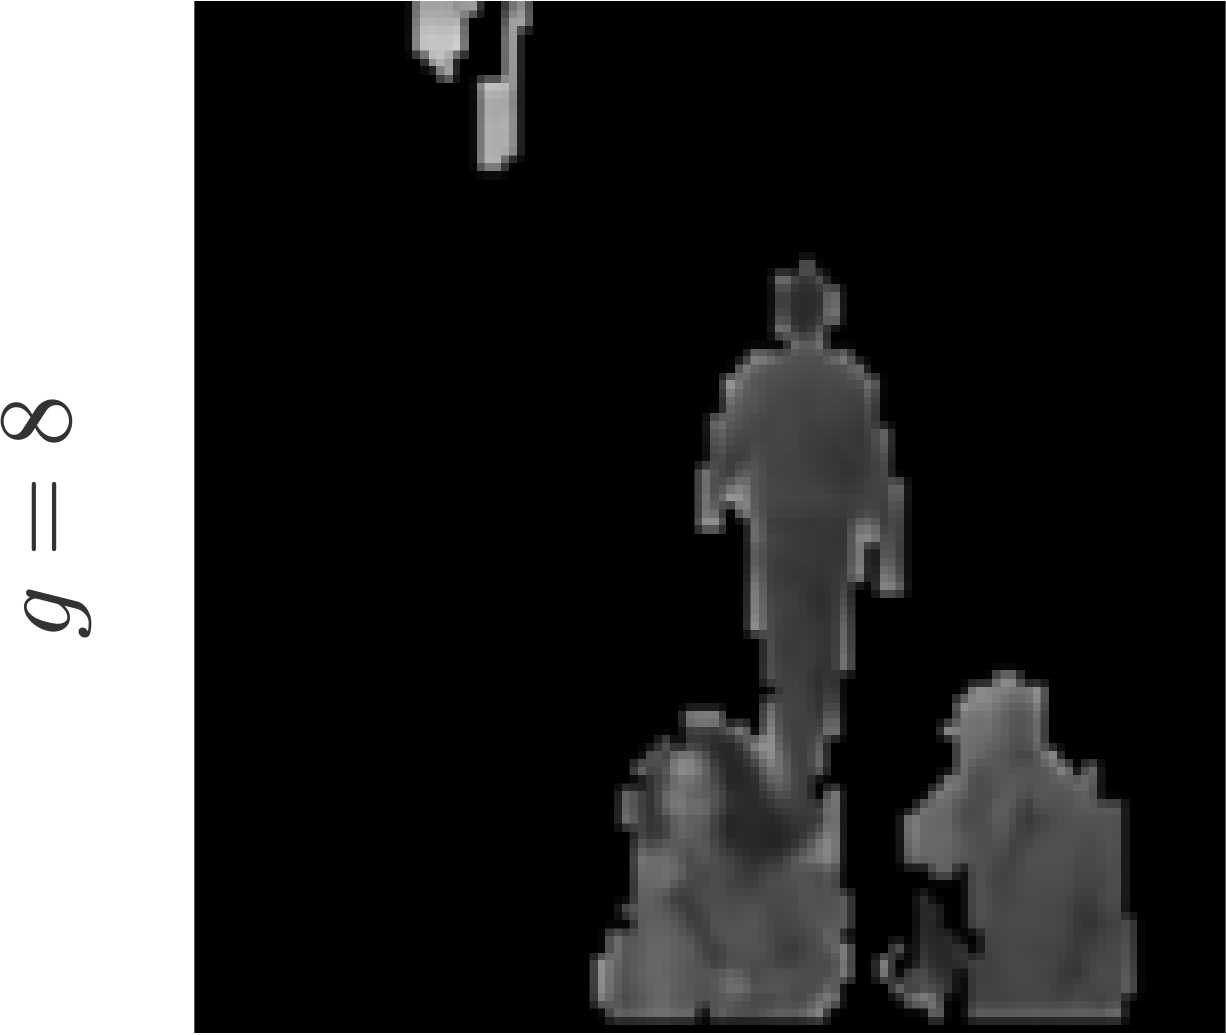}
	\includegraphics[width = 0.15\linewidth]{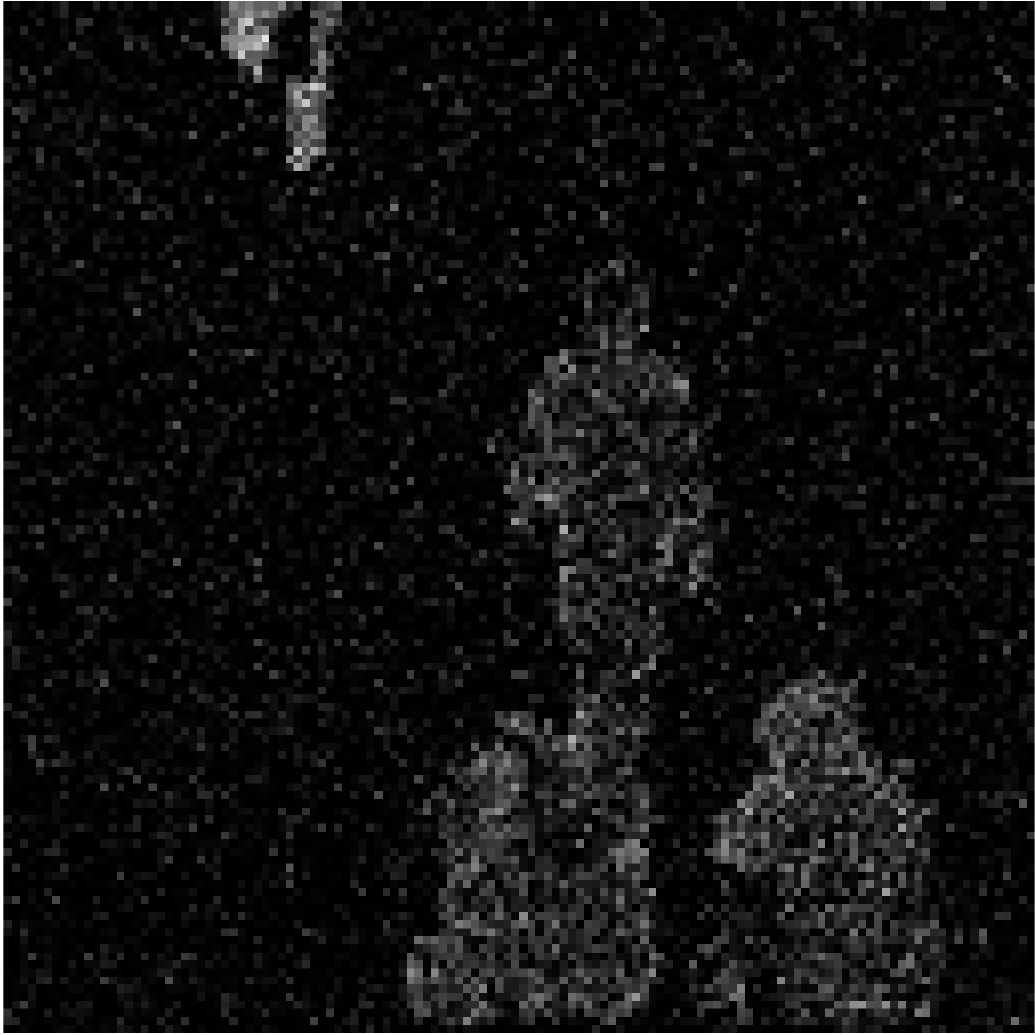}
	\includegraphics[width = 0.15\linewidth]{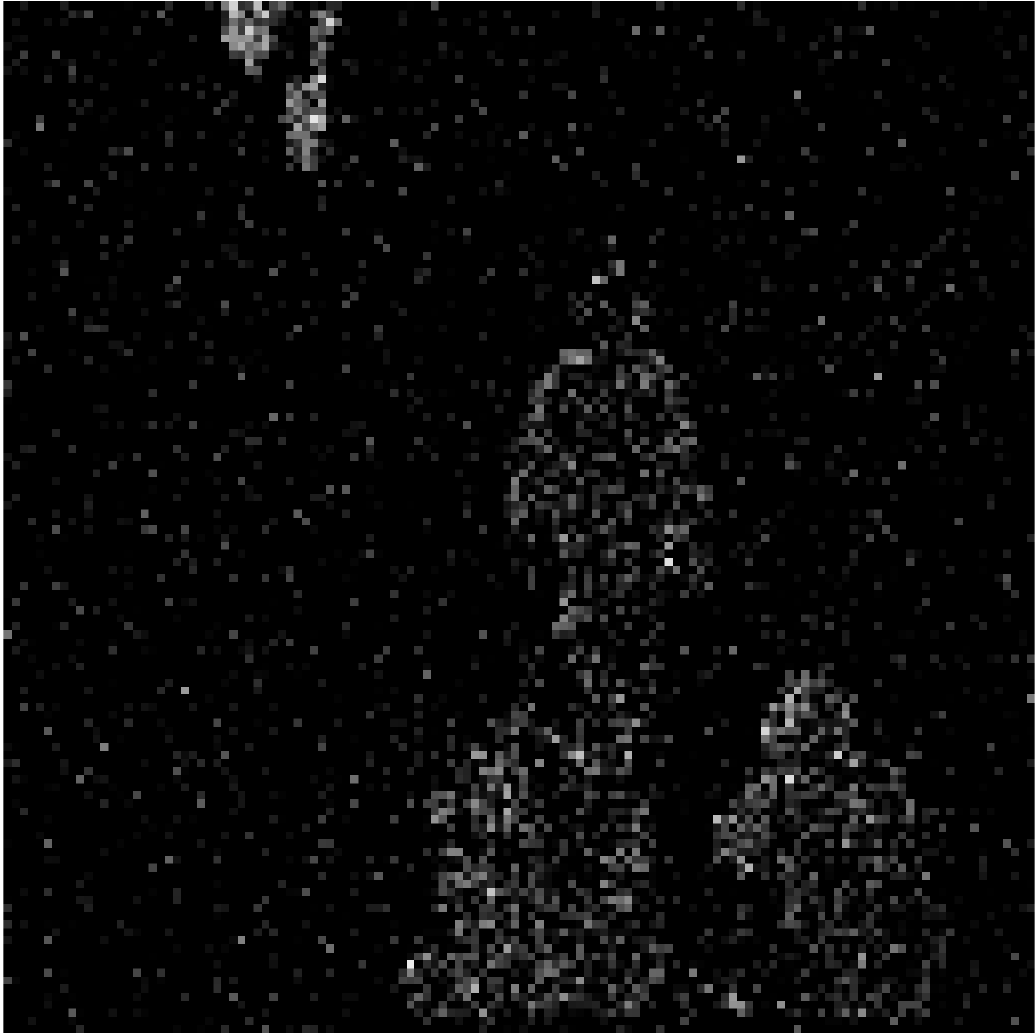}
	\includegraphics[width = 0.15\linewidth]{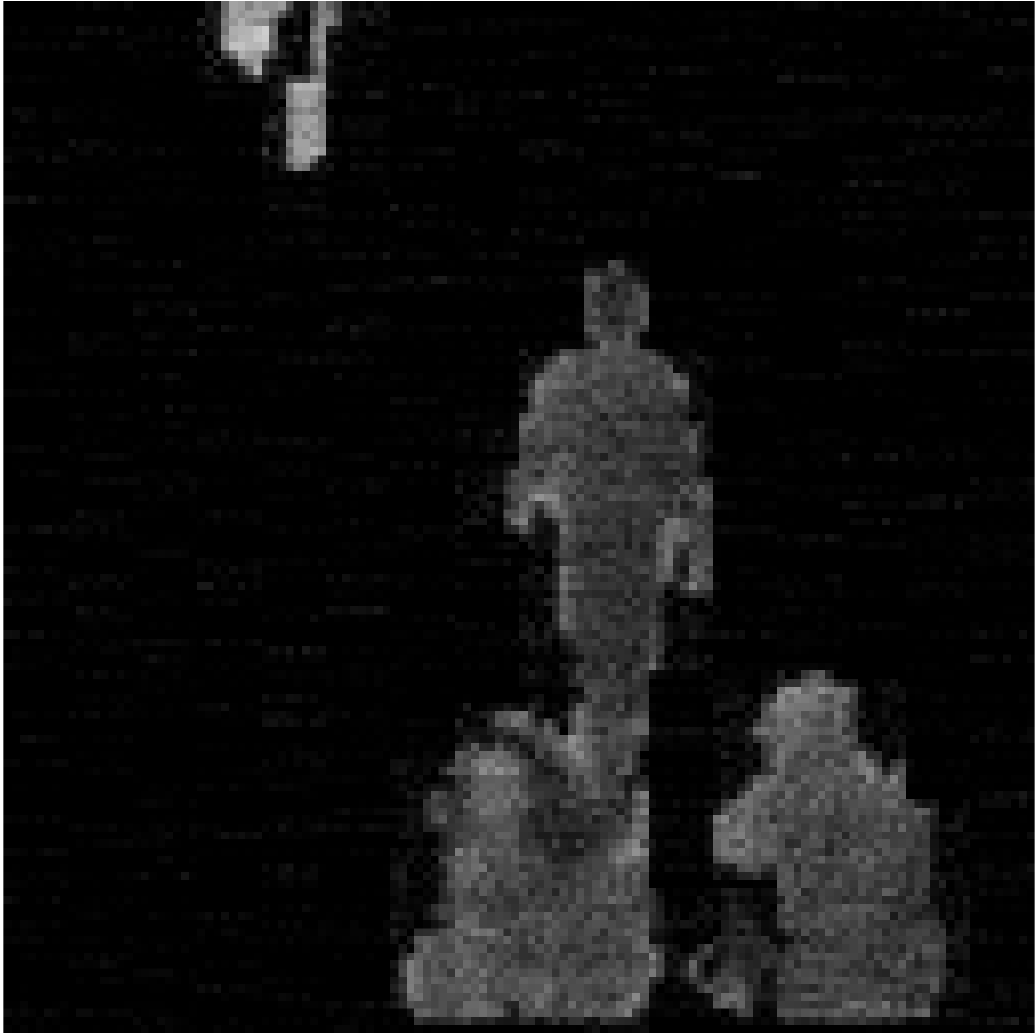}
	\includegraphics[width = 0.15\linewidth]{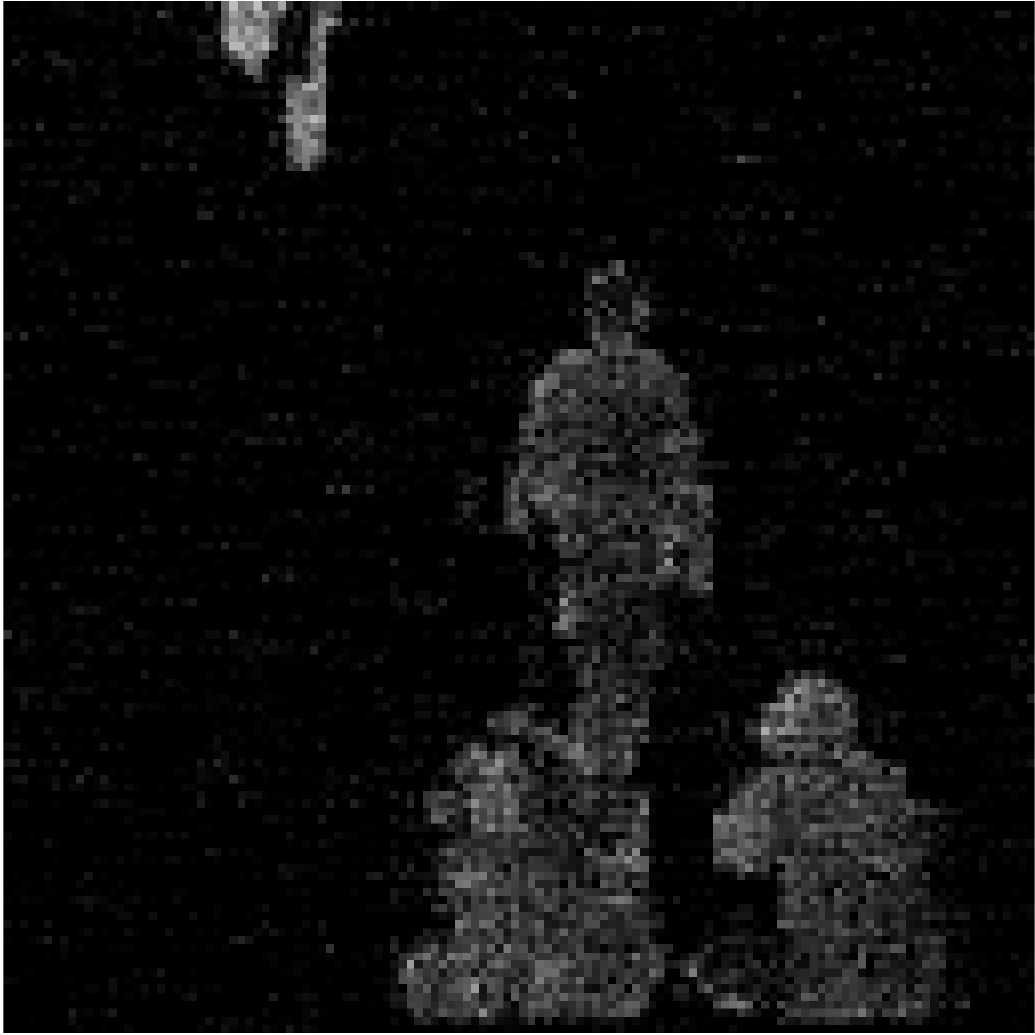} \vspace{-2mm} \\
	\begin{minipage}{0.15\linewidth}
	\centering  \small{$\phantom{a}$}
	\end{minipage}	
	\begin{minipage}{0.15\linewidth}
	\centering  \small{$20.6 ~\rm{dB}$}
	\end{minipage}
	\begin{minipage}{0.15\linewidth}
	\centering \small{$18.4 ~\rm{dB}$}
	\end{minipage}
	\begin{minipage}{0.15\linewidth}
	\centering \small{$30.8 ~\rm{dB}$}
	\end{minipage}
	\begin{minipage}{0.15\linewidth}
	\centering \small{$23.3 ~\rm{dB}$}
	\end{minipage}\\
	\includegraphics[width = 0.18\linewidth]{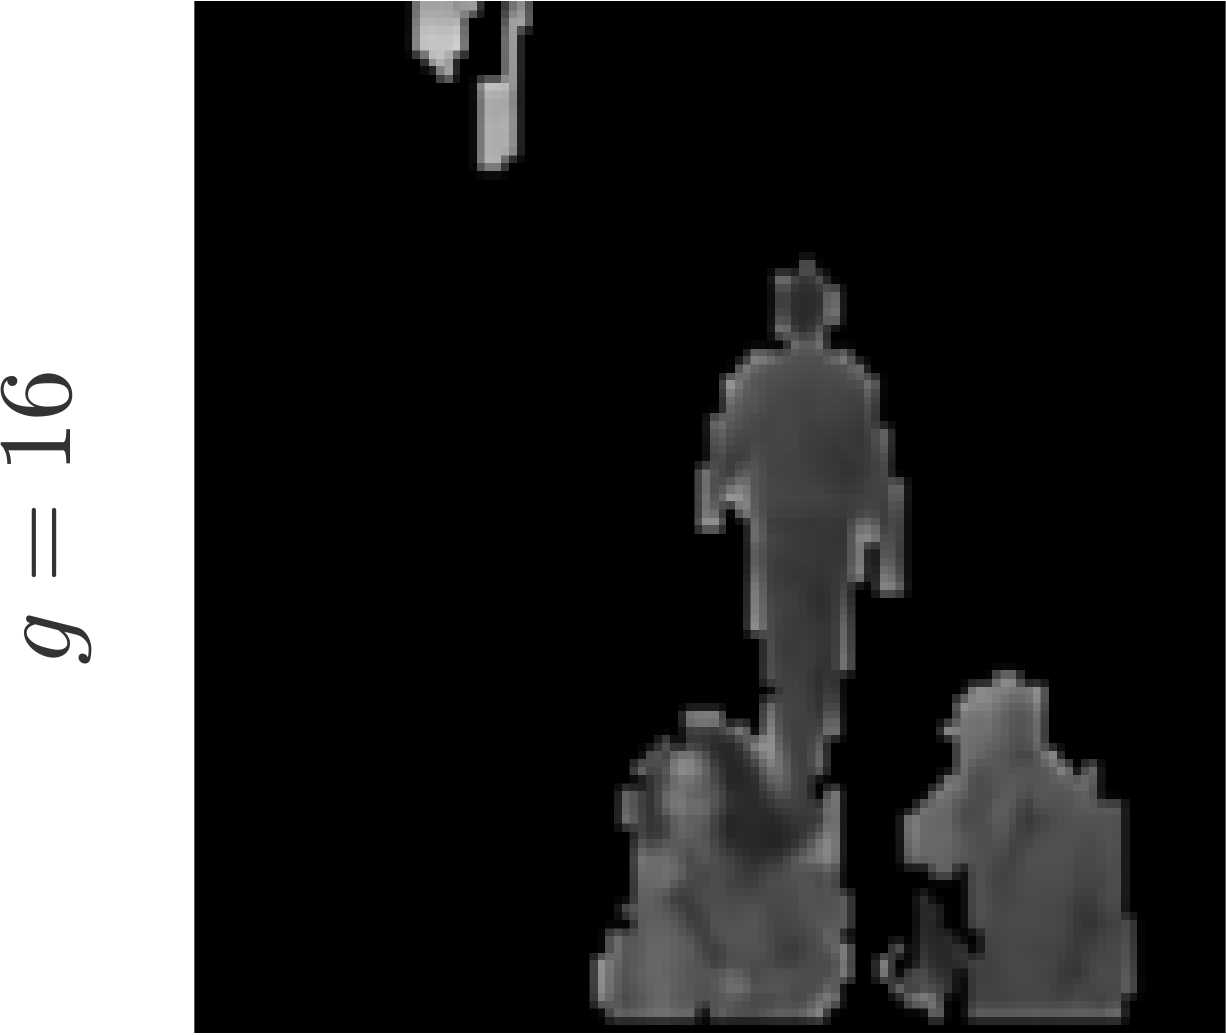}
	\includegraphics[width = 0.15\linewidth]{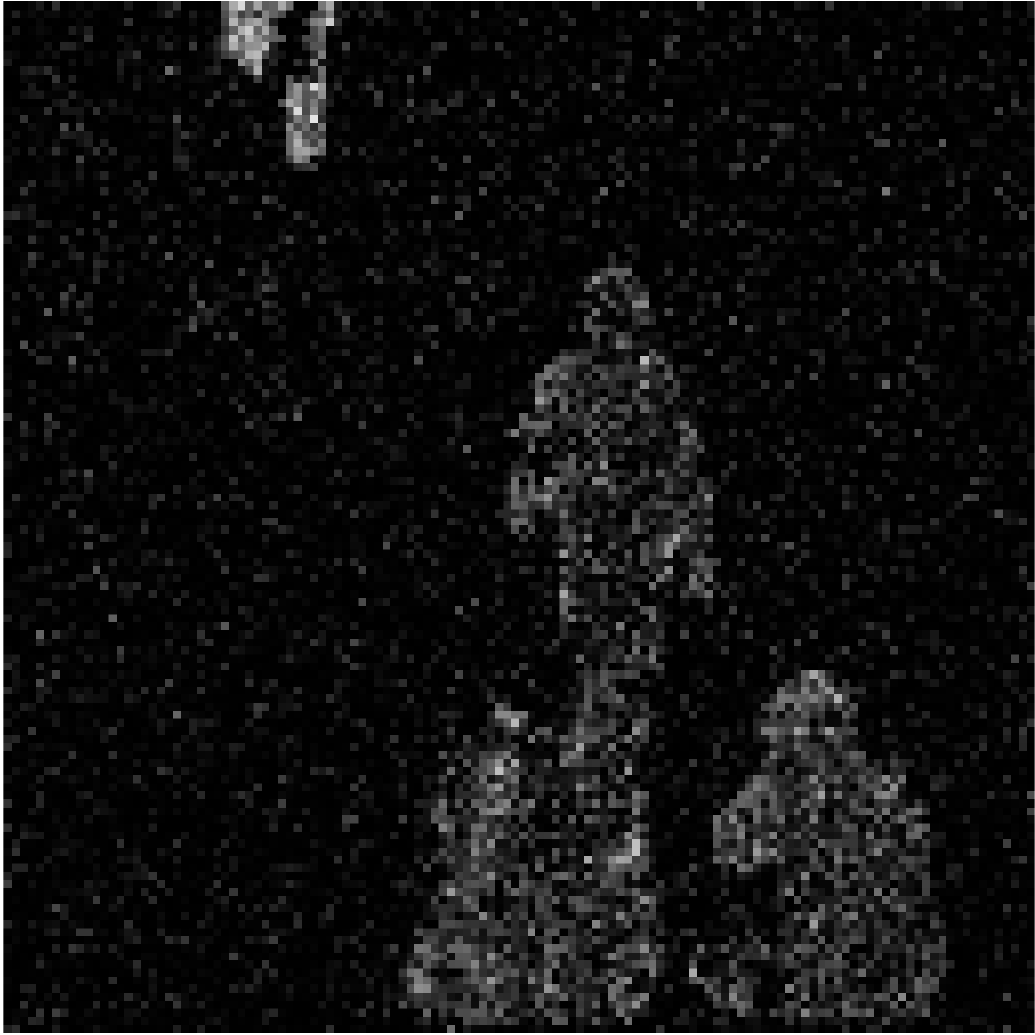}
	\includegraphics[width = 0.15\linewidth]{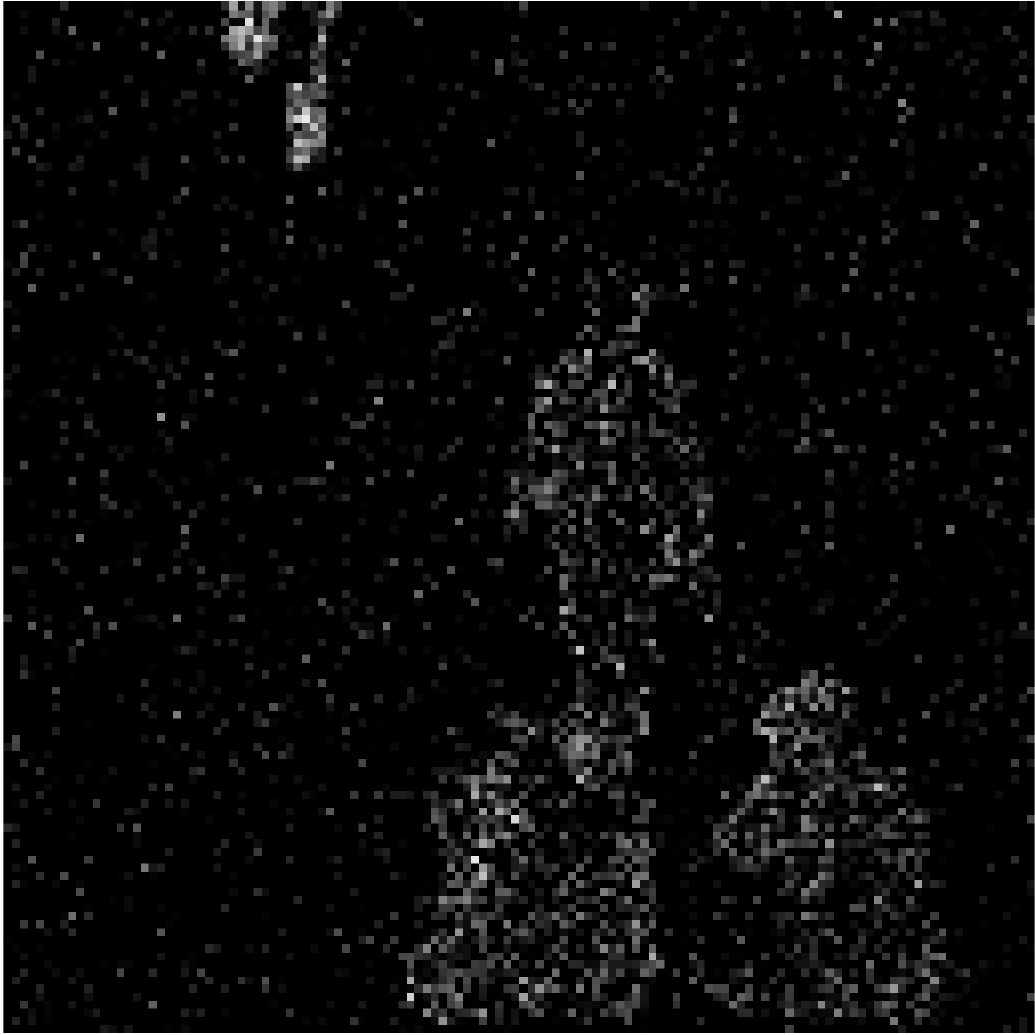}
	\includegraphics[width = 0.15\linewidth]{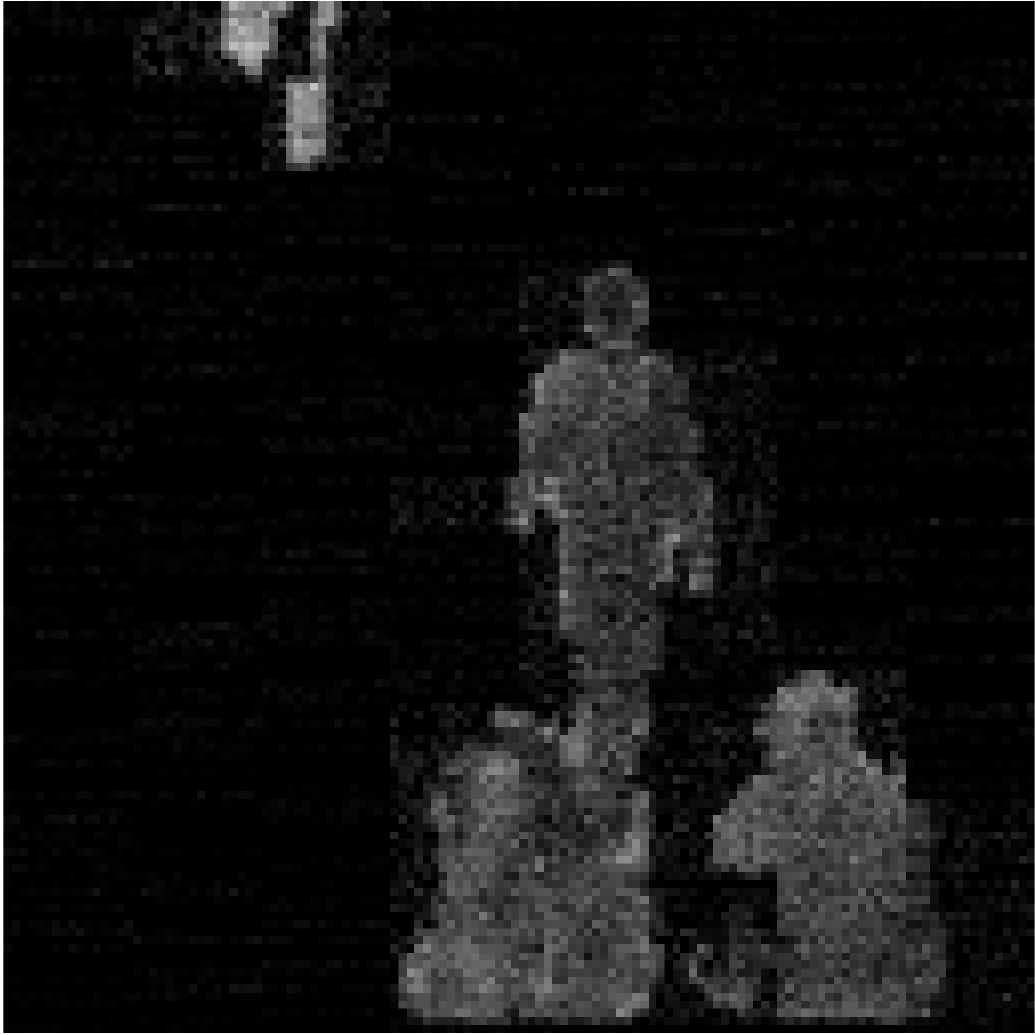}
	\includegraphics[width = 0.15\linewidth]{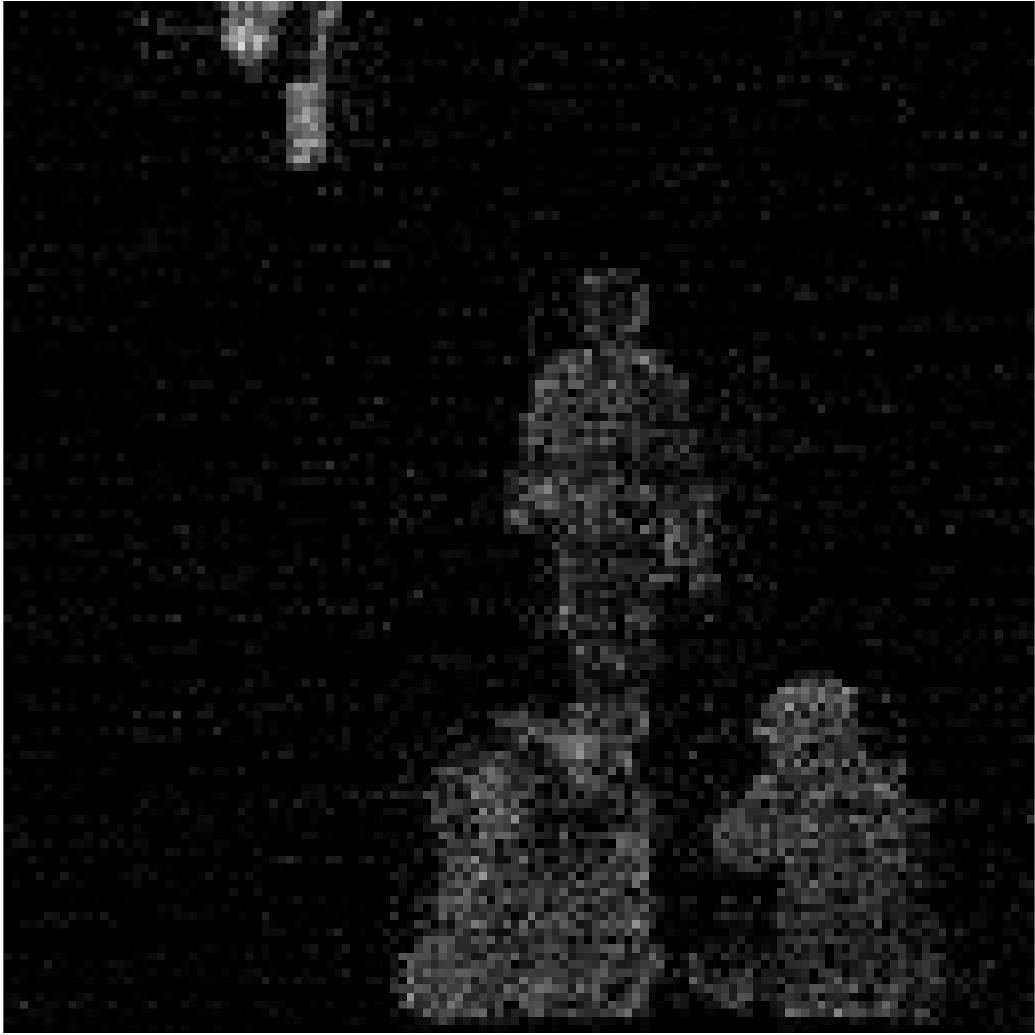} \vspace{-2mm} \\
	\begin{minipage}{0.15\linewidth}
	\centering  \small{$\phantom{a}$}
	\end{minipage}	
	\begin{minipage}{0.15\linewidth}
	\centering  \small{$20.7 ~\rm{dB}$}
	\end{minipage}
	\begin{minipage}{0.15\linewidth}
	\centering \small{$18.5 ~\rm{dB}$}
	\end{minipage}
	\begin{minipage}{0.15\linewidth}
	\centering \small{$28.0 ~\rm{dB}$}
	\end{minipage}
	\begin{minipage}{0.15\linewidth}
	\centering \small{$22.2 ~\rm{dB}$}
	\end{minipage} 

\caption{Results from real data. Reprentative examples of subtracted frame recovery from compressed measurements. Here,  $\numsam = \lceil 0.3 \cdot \dim \rceil $ measurements are observed for $\dim = 2^{14}$. From top to bottom, each line corresponds to block sparse model $\model$ with groups of consecutive indices, where $g = 4$, $g = 8$, and $g = 16$, respectively. One can observe that one obtains worse recovery as the group size increases; thus a model with groups $g = 4$ is a good choice for this case. } {\label{fig:003}}
\end{figure*}

\begin{figure*}[b]
\centering
	\begin{minipage}{0.15\linewidth}
	\centering \small{Original}
	\end{minipage}
	\begin{minipage}{0.15\linewidth}
	\centering \small{$\ell_1$ + Exp.}
	\end{minipage}
	\begin{minipage}{0.15\linewidth}
	\centering \small{$\ell_1$ + Gaus.}
	\end{minipage}
	\begin{minipage}{0.15\linewidth}
	\centering \small{$\ell_{2,1}$ + Exp.}
	\end{minipage}
	\begin{minipage}{0.15\linewidth}
	\centering \small{$\ell_{2,1}$ + Gaus.}
	\end{minipage}\\
	\includegraphics[width = 0.18\linewidth]{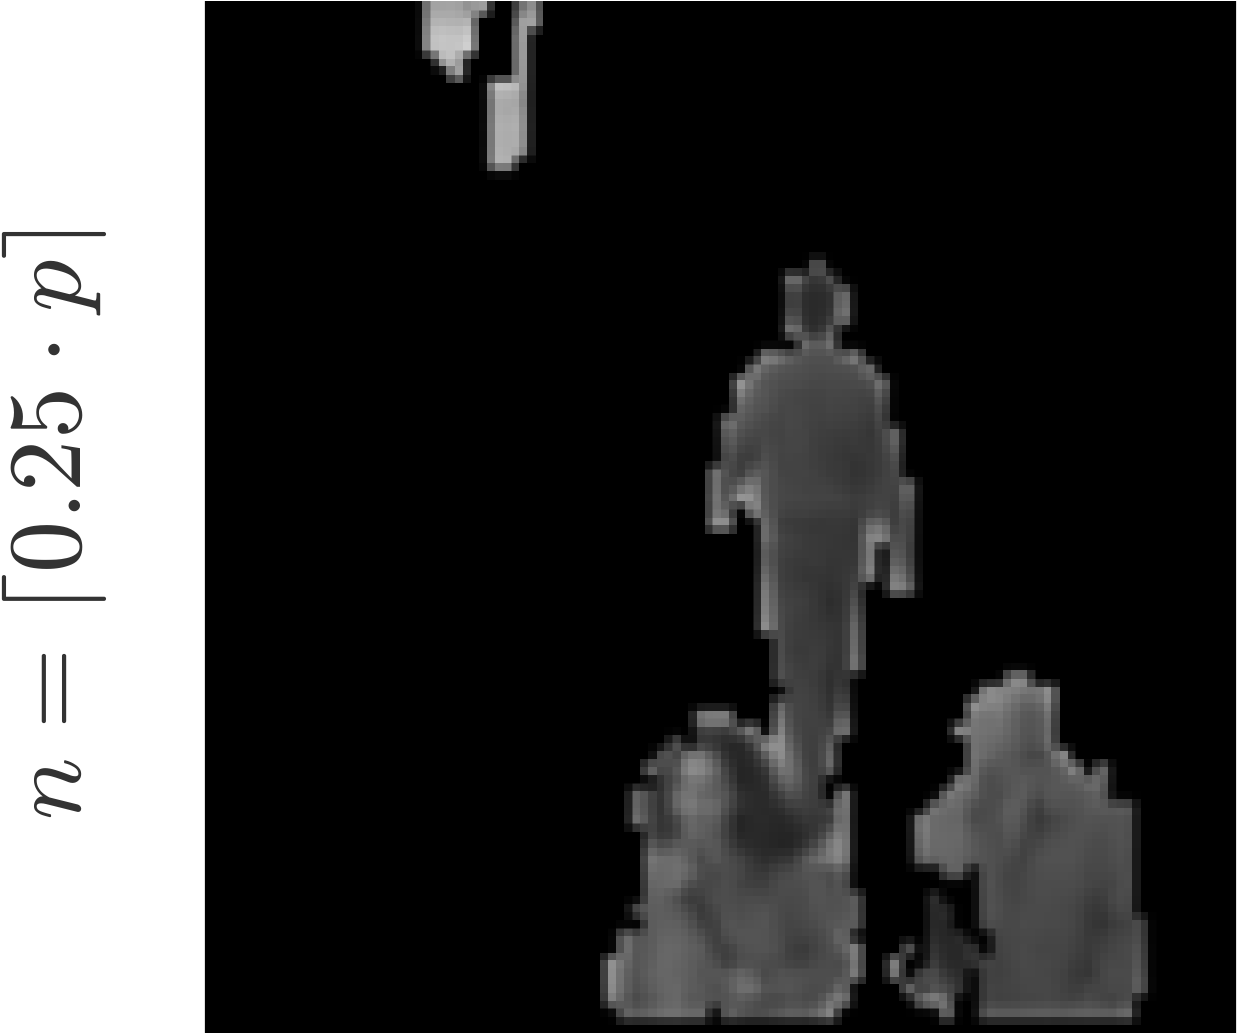}
	\includegraphics[width = 0.15\linewidth]{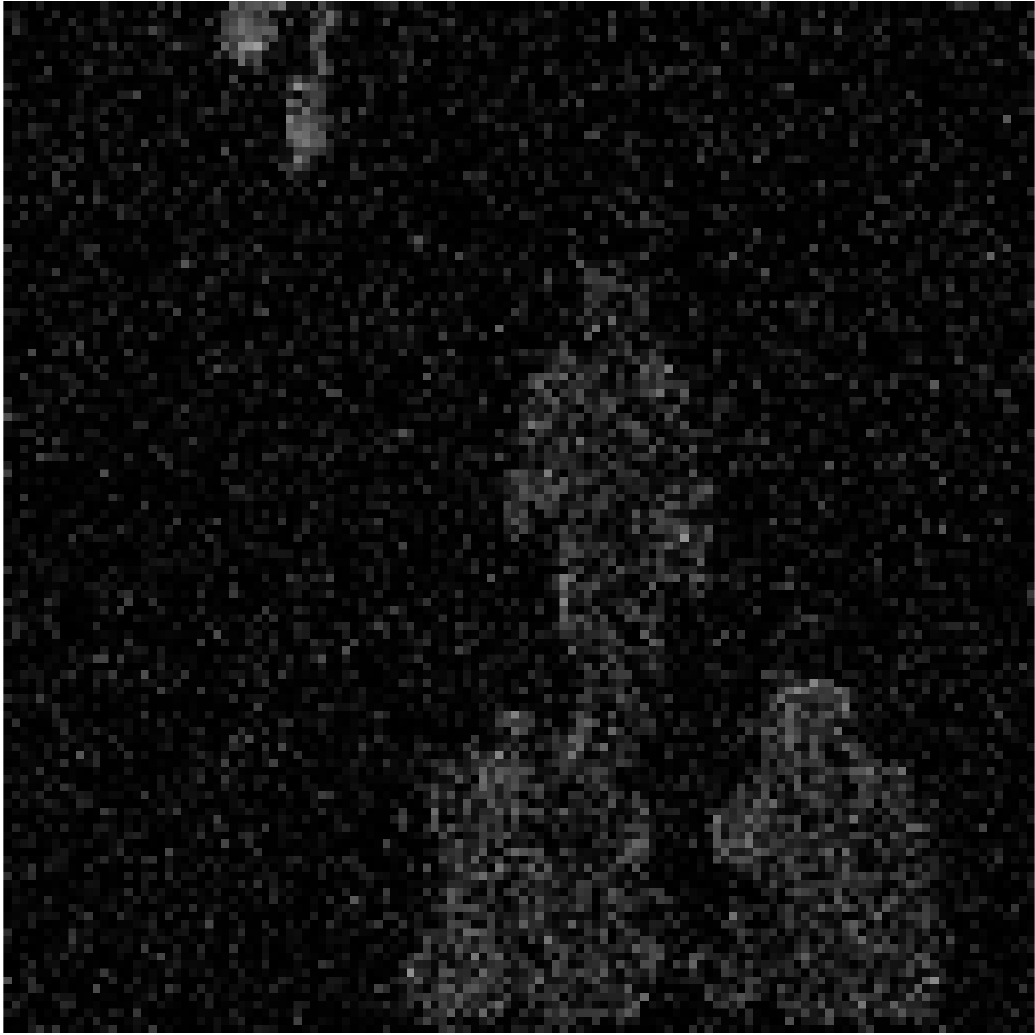}
	\includegraphics[width = 0.15\linewidth]{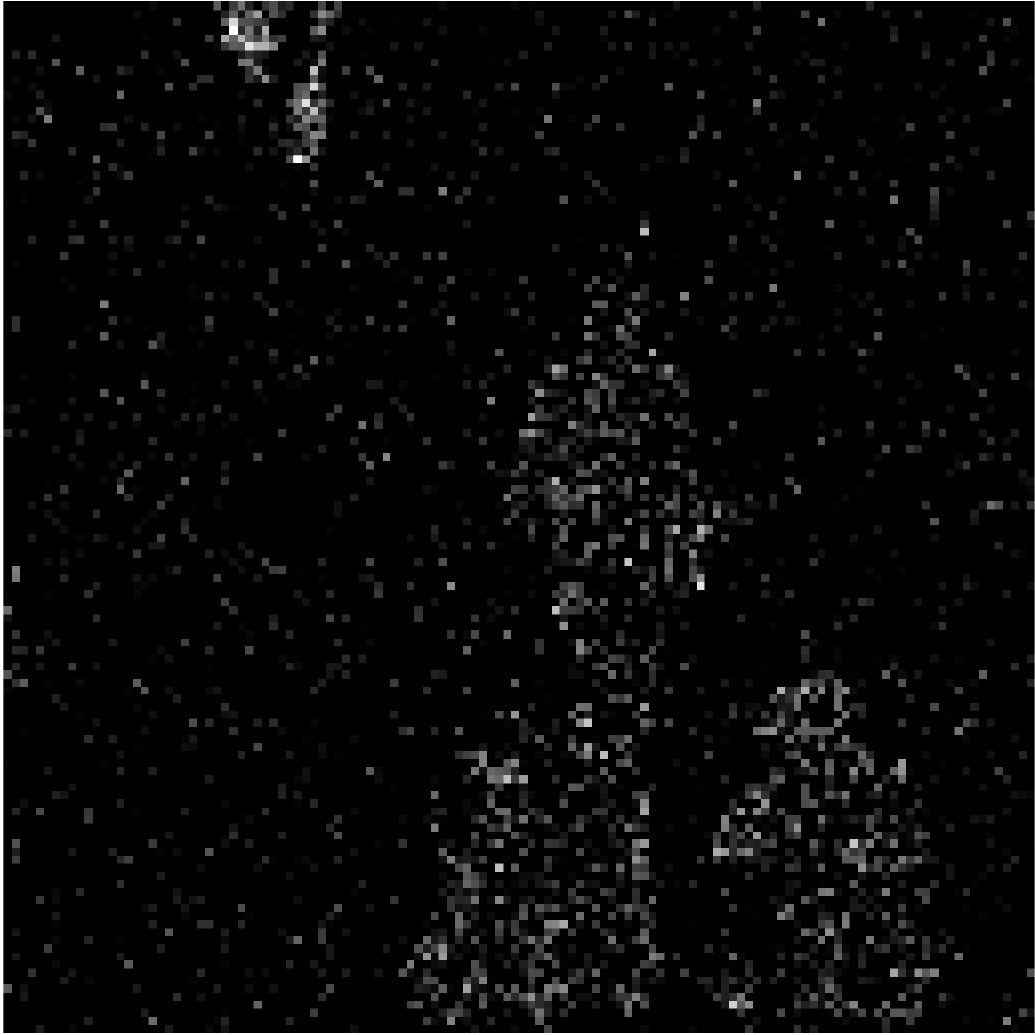}
	\includegraphics[width = 0.15\linewidth]{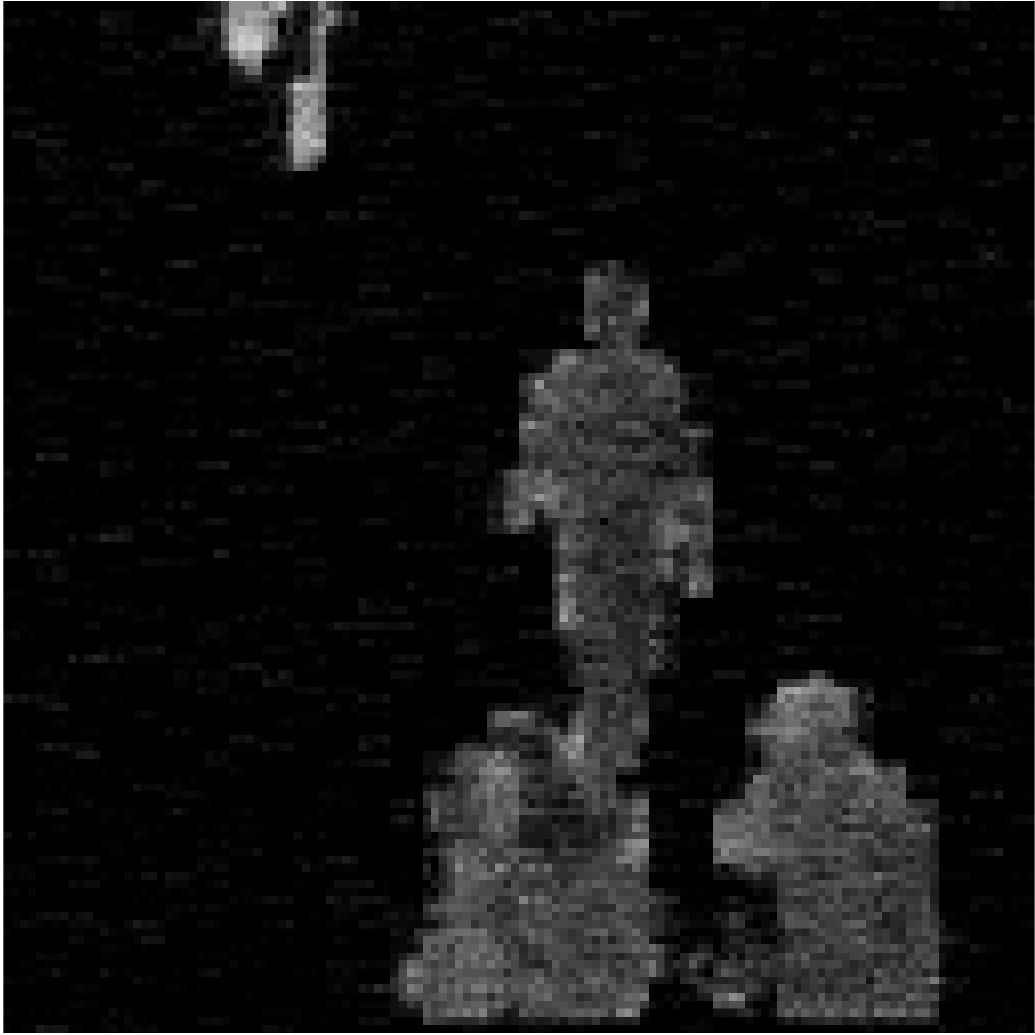}
	\includegraphics[width = 0.15\linewidth]{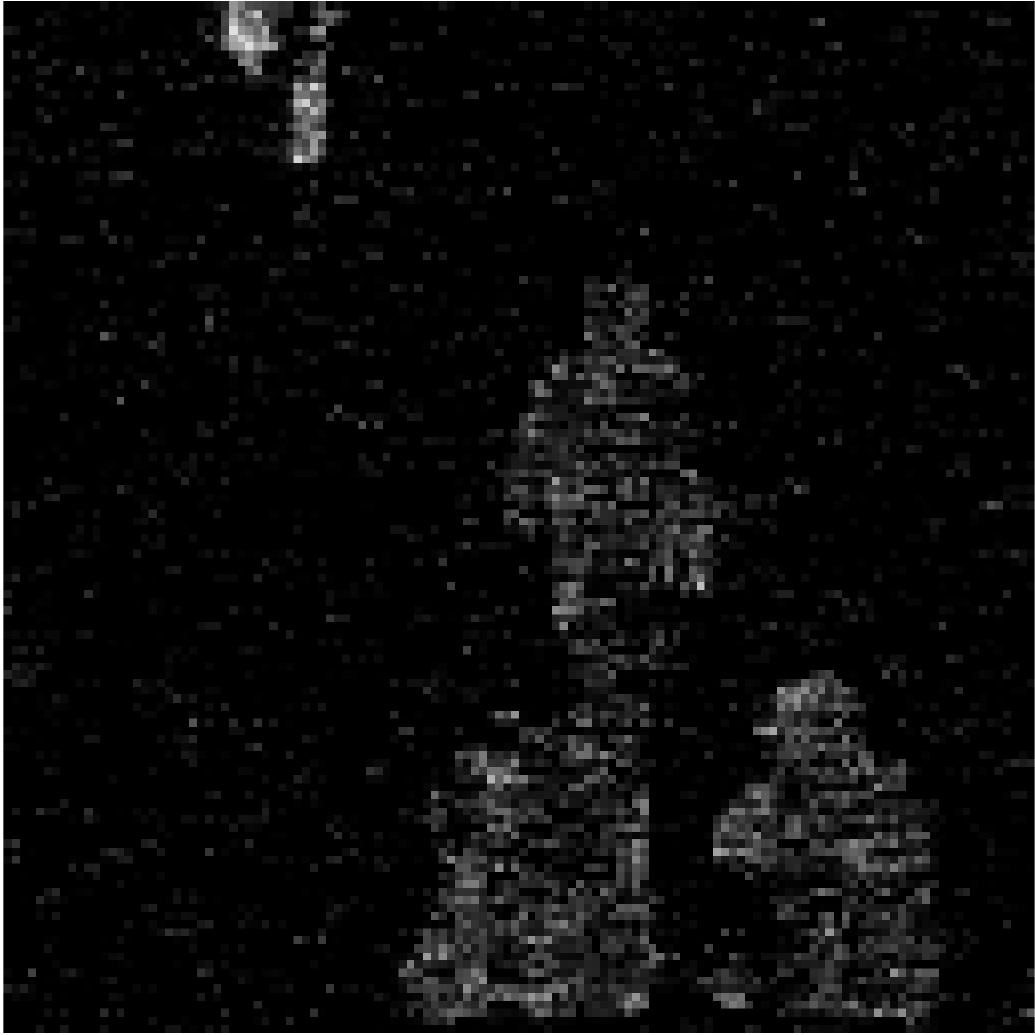} \vspace{-2mm} \\	
	\begin{minipage}{0.15\linewidth}
	\centering  \small{$\phantom{a}$}
	\end{minipage}	
	\begin{minipage}{0.15\linewidth}
	\centering  \small{$19.8 ~\rm{dB}$}
	\end{minipage}
	\begin{minipage}{0.15\linewidth}
	\centering \small{$17.8 ~\rm{dB}$}
	\end{minipage}
	\begin{minipage}{0.15\linewidth}
	\centering \small{$29.0 ~\rm{dB}$}
	\end{minipage}
	\begin{minipage}{0.15\linewidth}
	\centering \small{$20.3 ~\rm{dB}$}
	\end{minipage}\\
	\includegraphics[width = 0.18\linewidth]{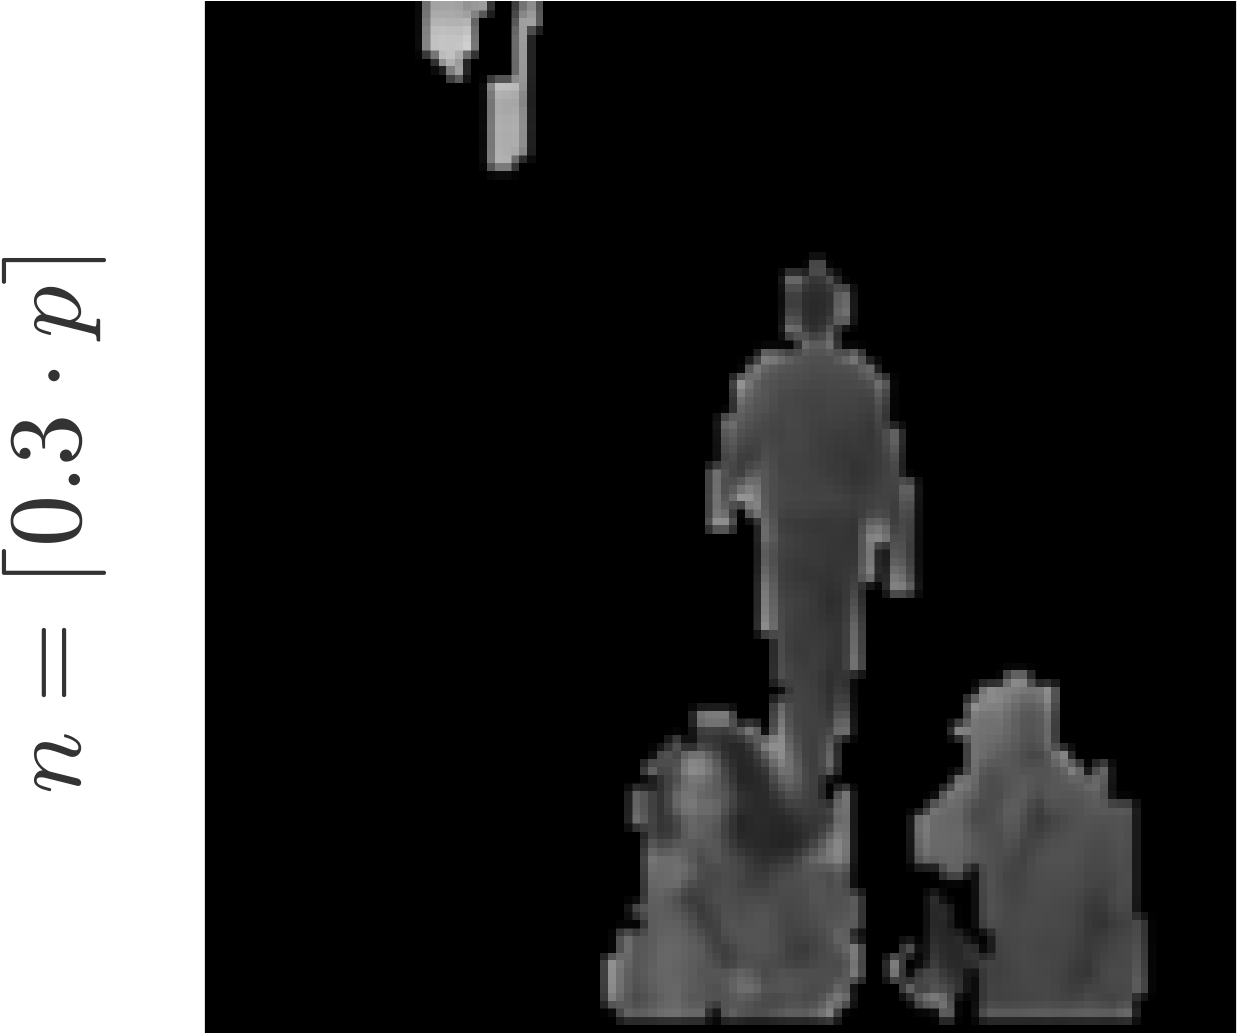}
	\includegraphics[width = 0.15\linewidth]{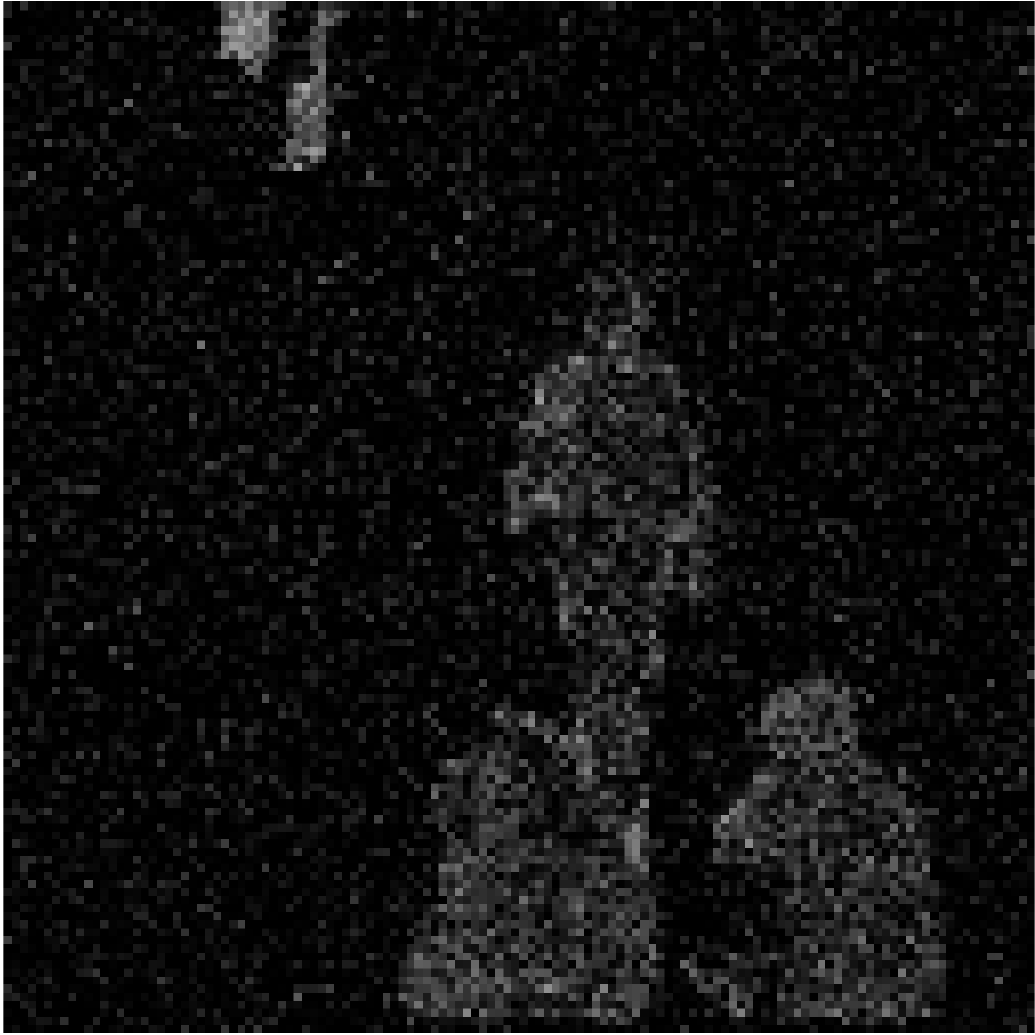}
	\includegraphics[width = 0.15\linewidth]{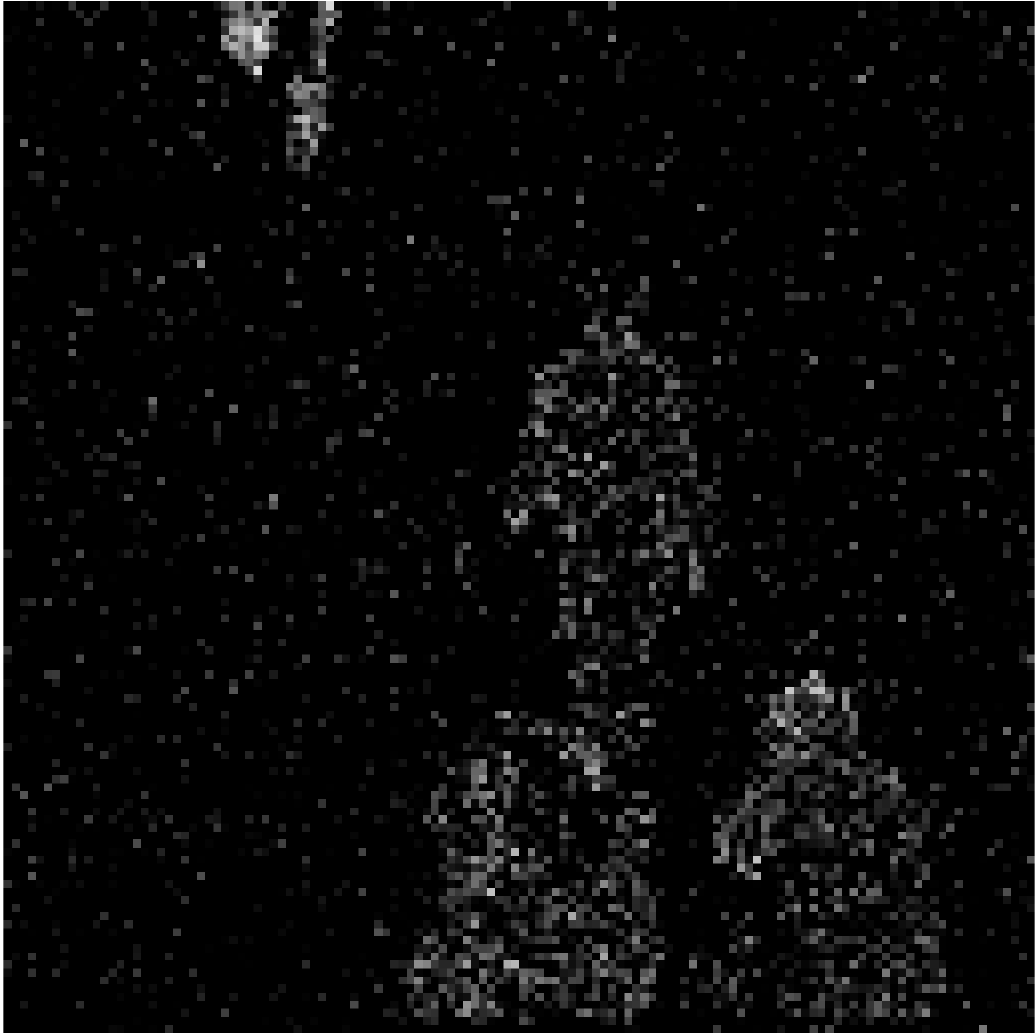}
	\includegraphics[width = 0.15\linewidth]{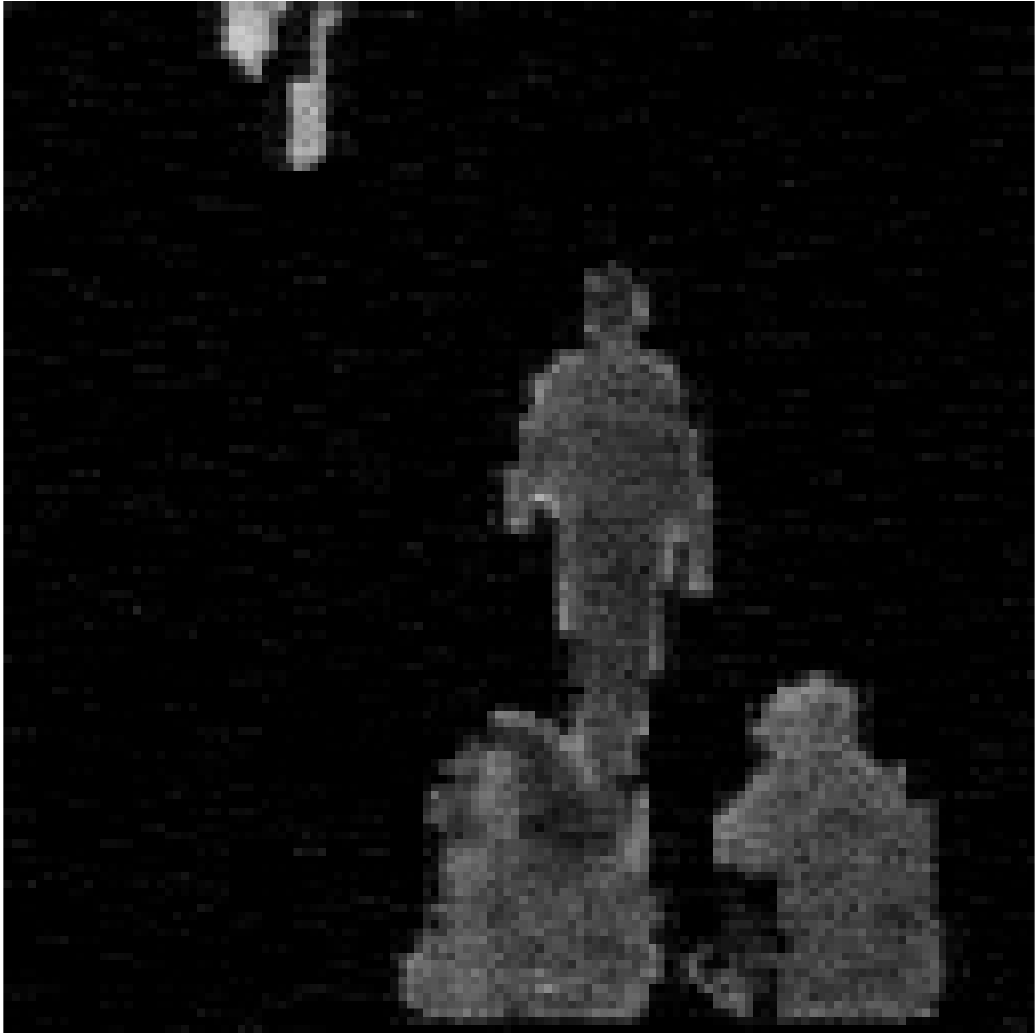}
	\includegraphics[width = 0.15\linewidth]{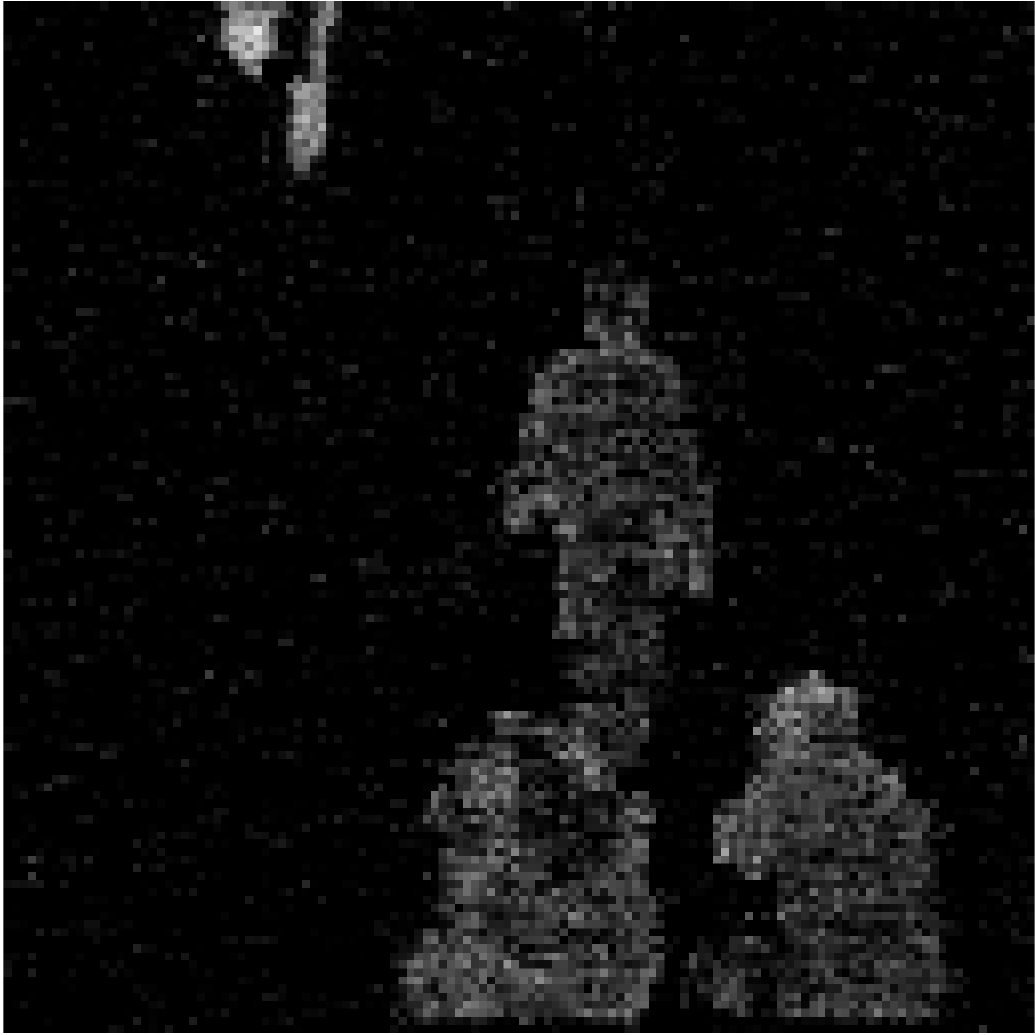} \vspace{-2mm} \\
	\begin{minipage}{0.15\linewidth}
	\centering  \small{$\phantom{a}$}
	\end{minipage}	
	\begin{minipage}{0.15\linewidth}
	\centering  \small{$20.6 ~\rm{dB}$}
	\end{minipage}
	\begin{minipage}{0.15\linewidth}
	\centering \small{$18.5 ~\rm{dB}$}
	\end{minipage}
	\begin{minipage}{0.15\linewidth}
	\centering \small{$31.5 ~\rm{dB}$}
	\end{minipage}
	\begin{minipage}{0.15\linewidth}
	\centering \small{$22.8 ~\rm{dB}$}
	\end{minipage}\\
	\includegraphics[width = 0.18\linewidth]{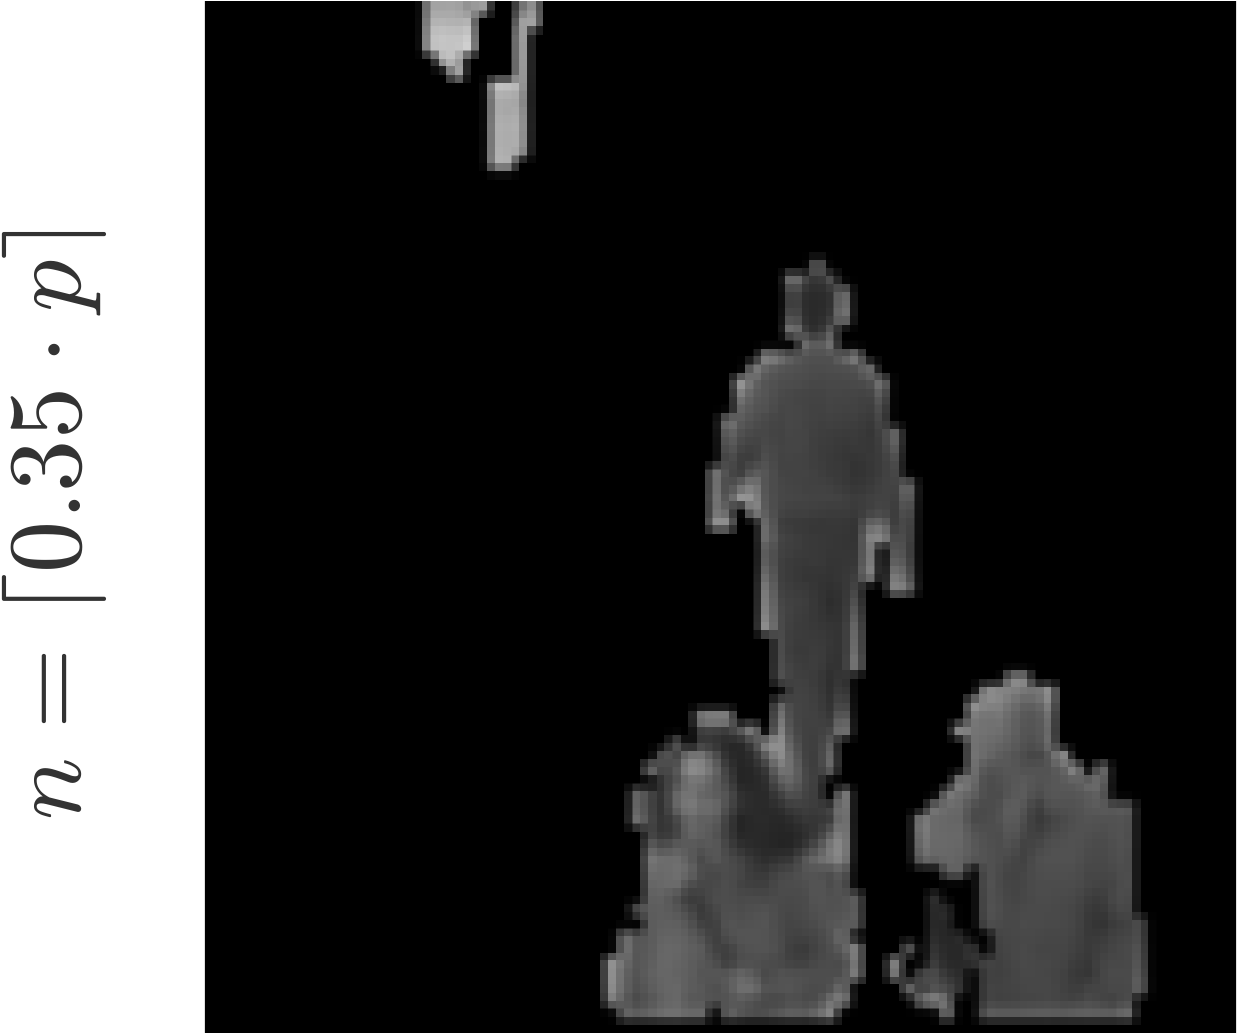}
	\includegraphics[width = 0.15\linewidth]{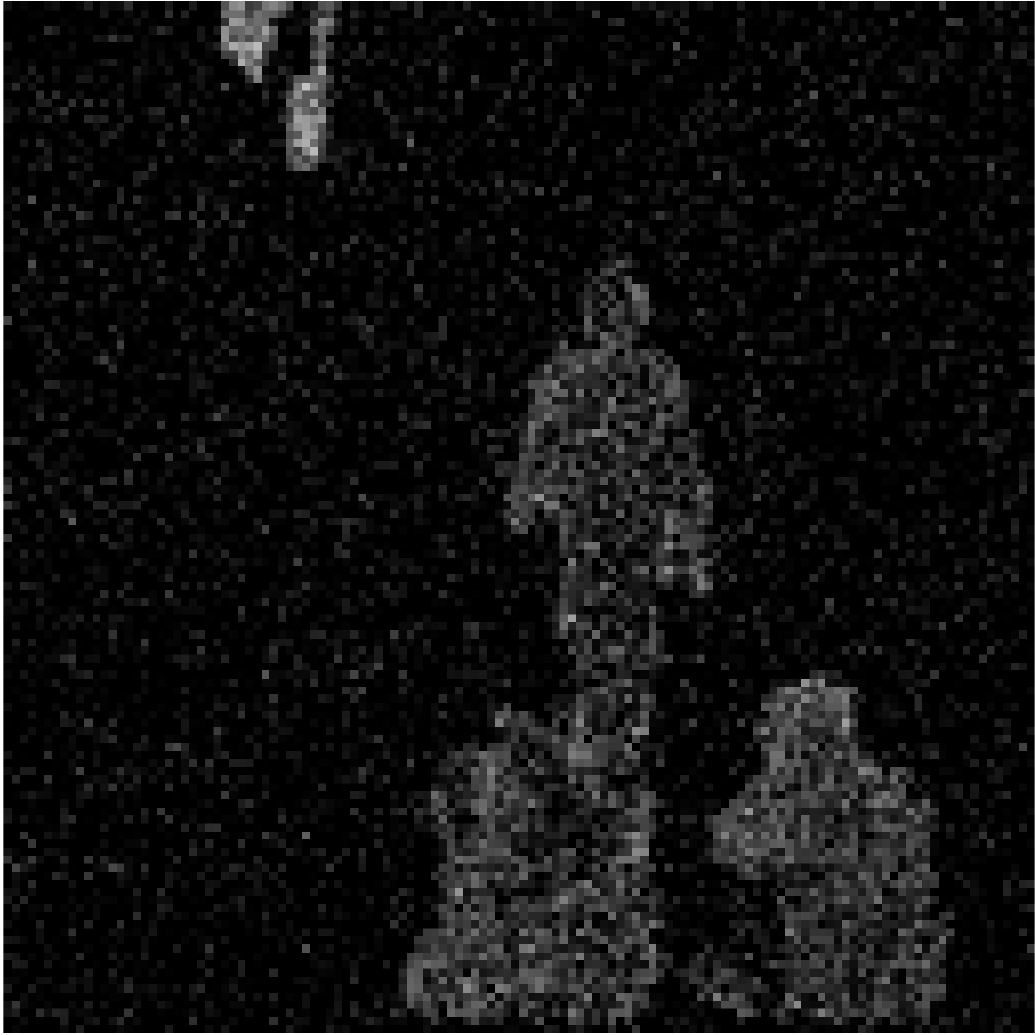}
	\includegraphics[width = 0.15\linewidth]{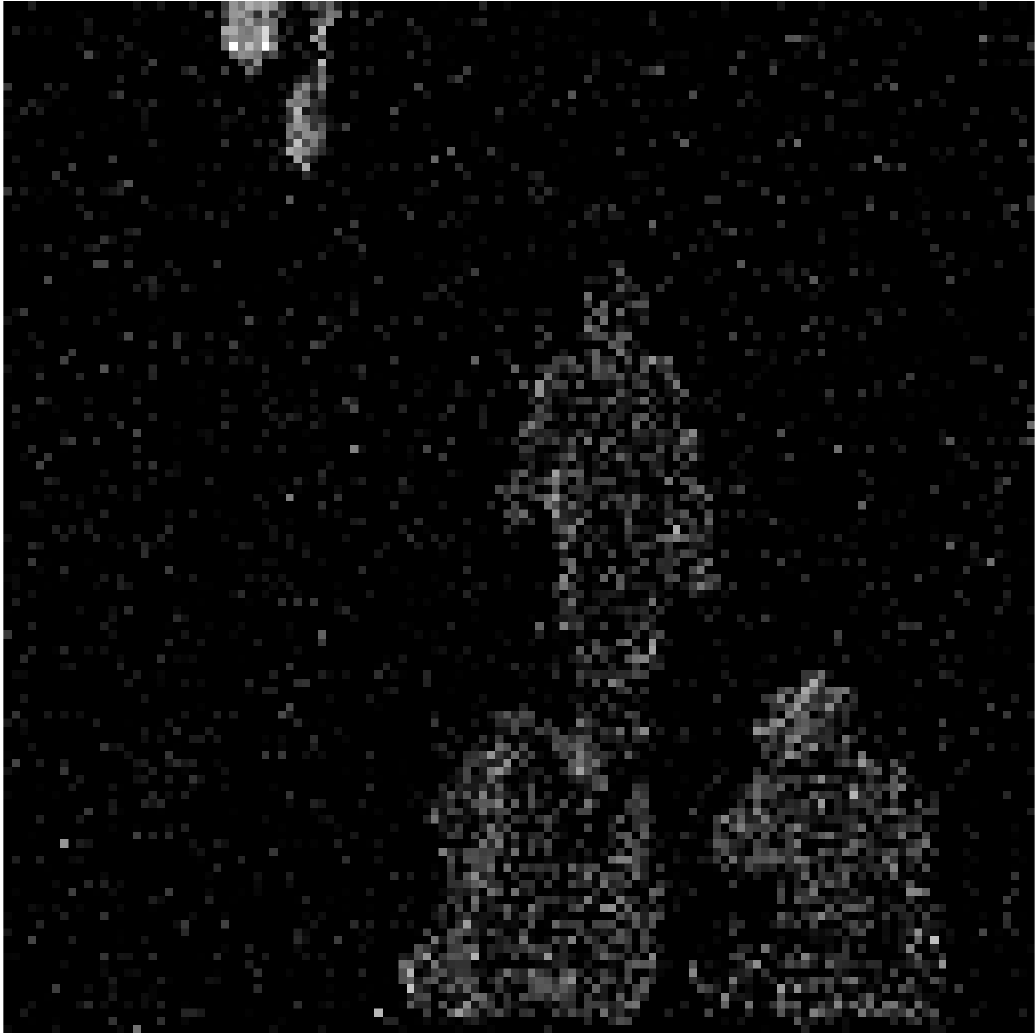}
	\includegraphics[width = 0.15\linewidth]{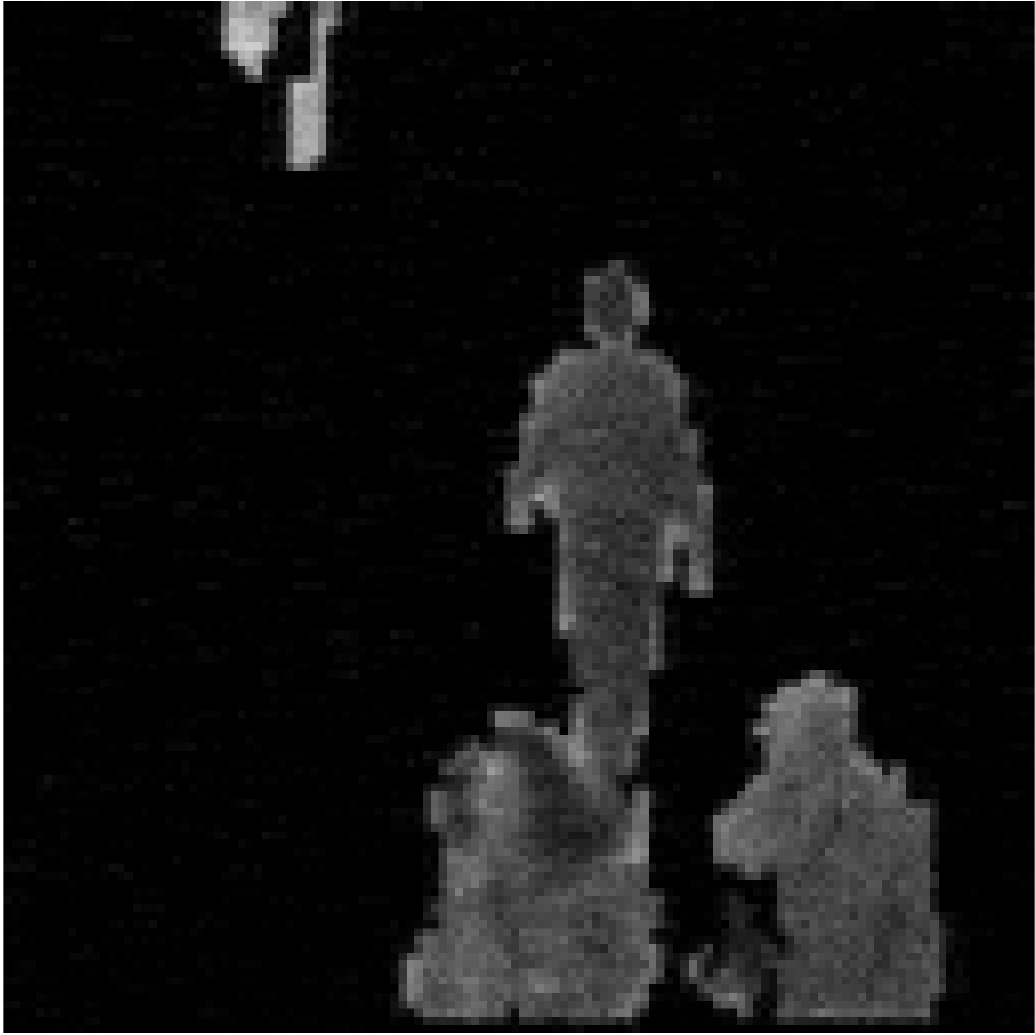}
	\includegraphics[width = 0.15\linewidth]{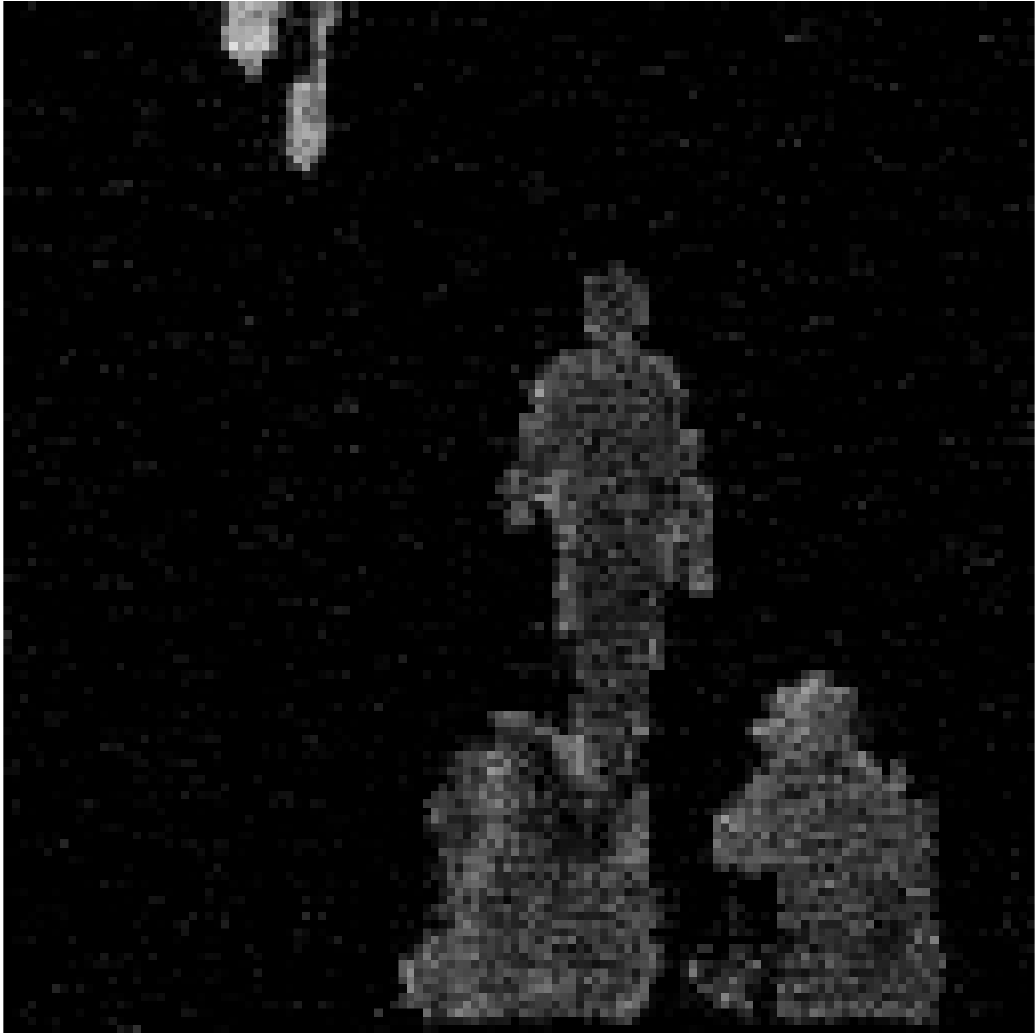} \vspace{-2mm} \\
	\begin{minipage}{0.15\linewidth}
	\centering  \small{$\phantom{a}$}
	\end{minipage}	
	\begin{minipage}{0.15\linewidth}
	\centering  \small{$21.7 ~\rm{dB}$}
	\end{minipage}
	\begin{minipage}{0.15\linewidth}
	\centering \small{$19.3~\rm{dB}$}
	\end{minipage}
	\begin{minipage}{0.15\linewidth}
	\centering \small{$34.9 ~\rm{dB}$}
	\end{minipage}
	\begin{minipage}{0.15\linewidth}
	\centering \small{$25.3 ~\rm{dB}$}
	\end{minipage} \\
	\includegraphics[width = 0.18\linewidth]{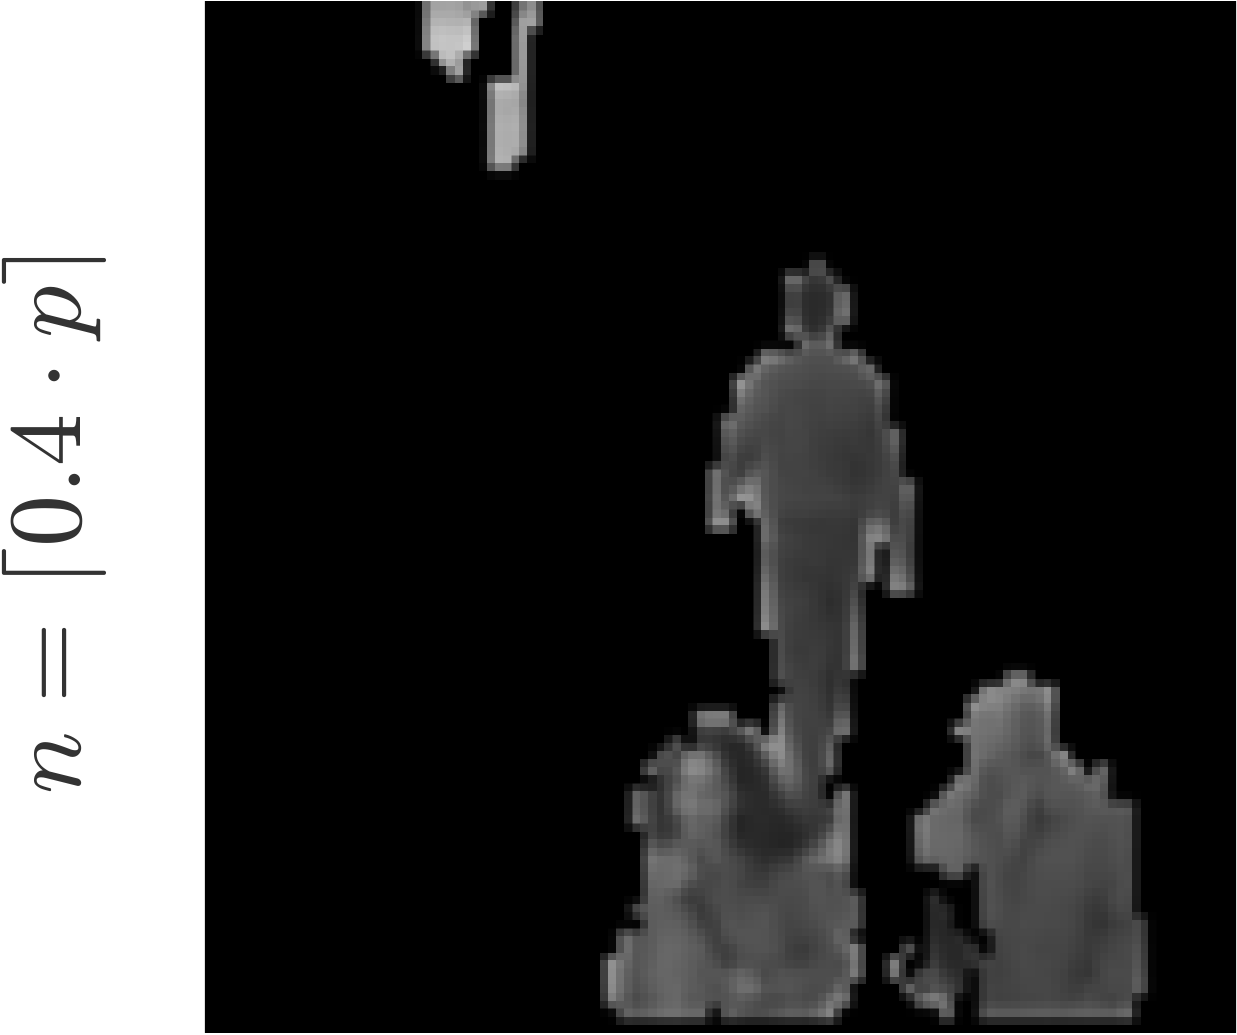}
	\includegraphics[width = 0.15\linewidth]{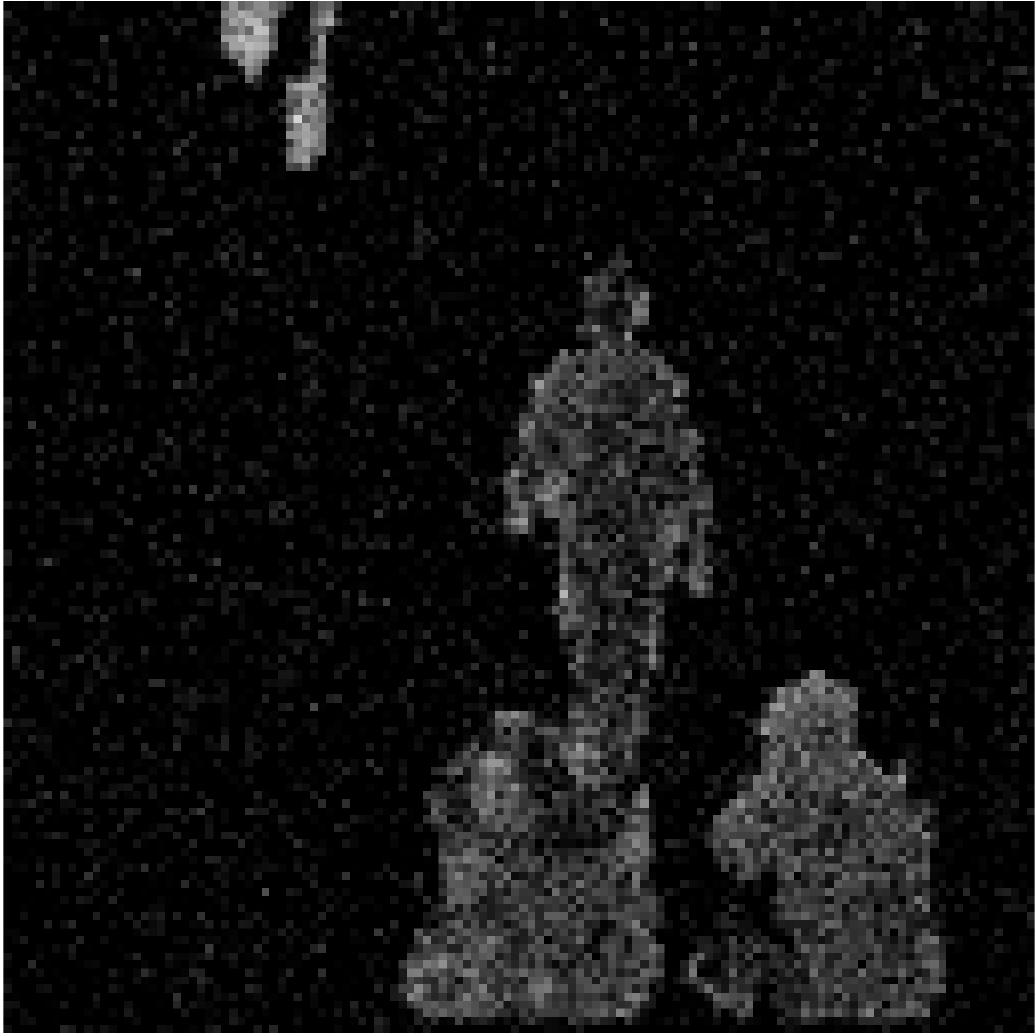}
	\includegraphics[width = 0.15\linewidth]{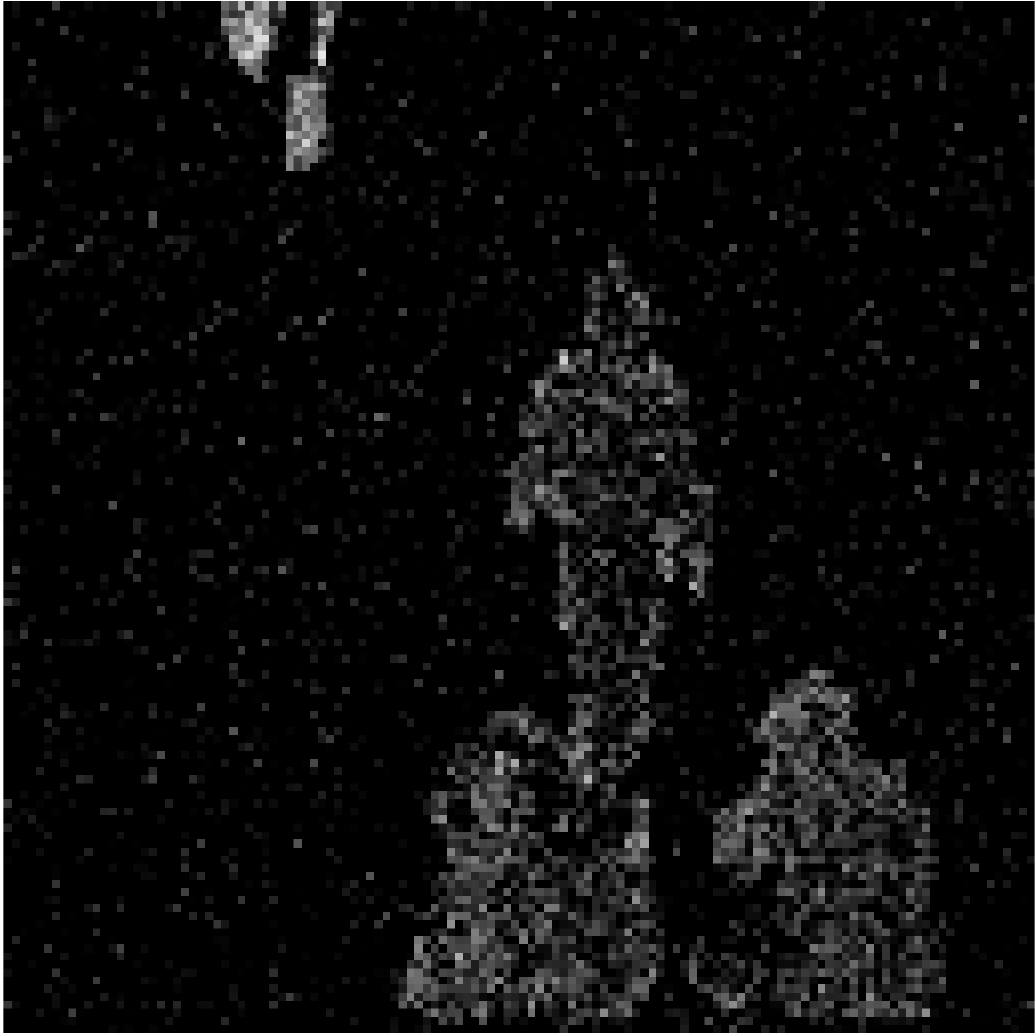}
	\includegraphics[width = 0.15\linewidth]{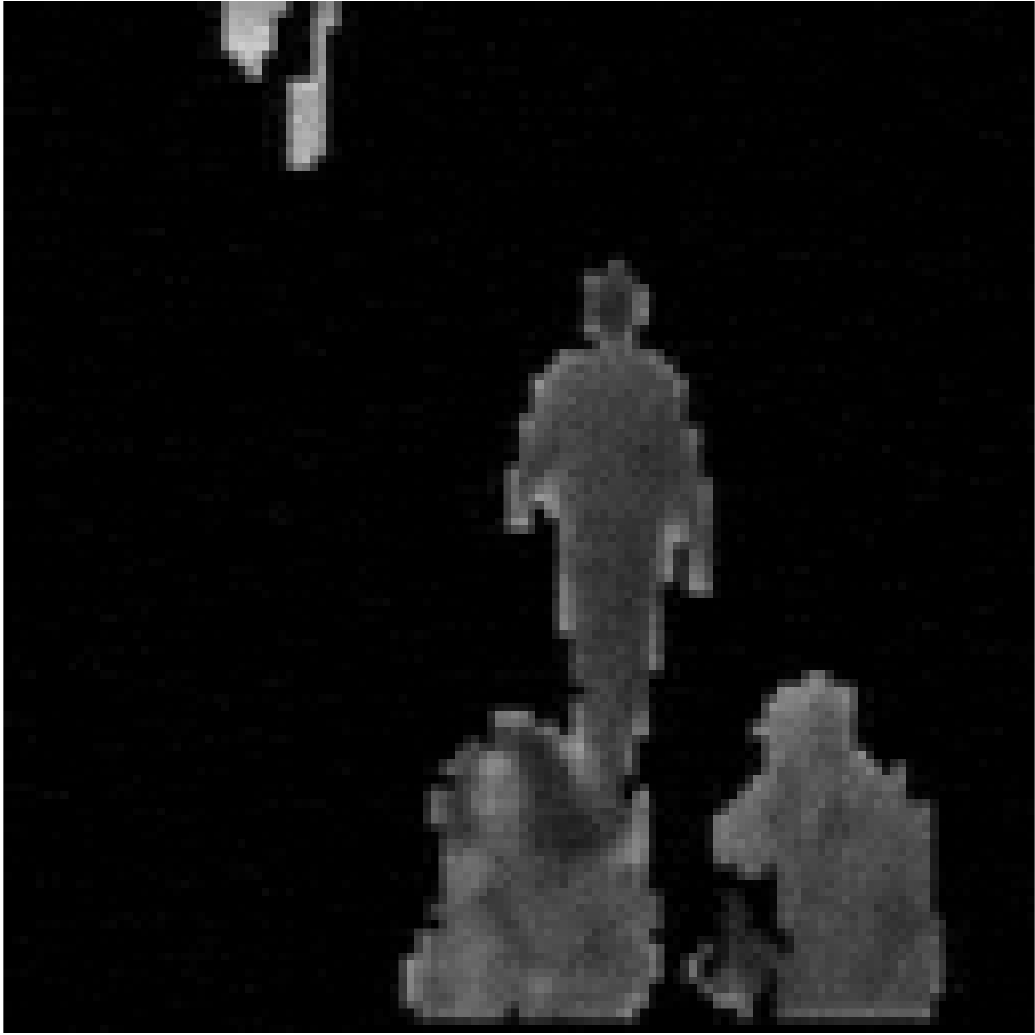}
	\includegraphics[width = 0.15\linewidth]{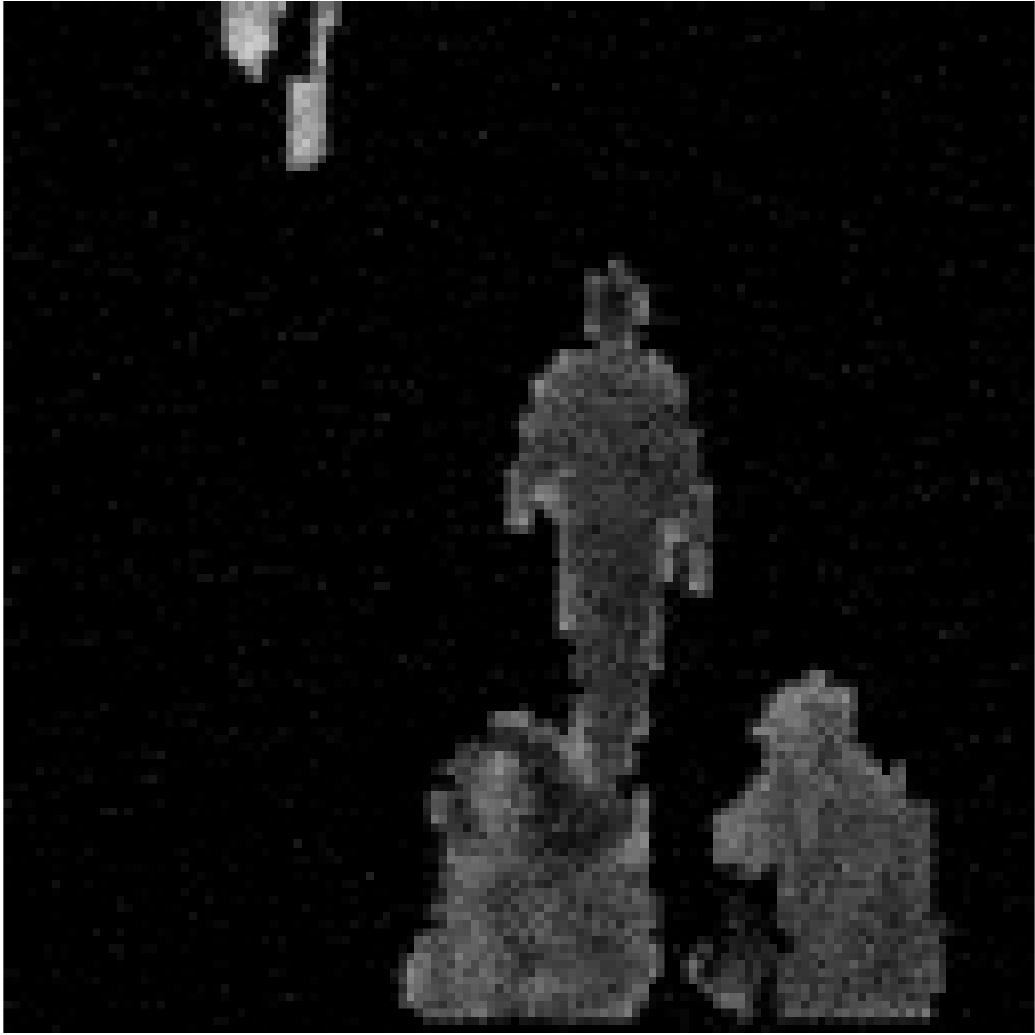} \vspace{-2mm} \\
	\begin{minipage}{0.15\linewidth}
	\centering  \small{$\phantom{a}$}
	\end{minipage}	
	\begin{minipage}{0.15\linewidth}
	\centering  \small{$23.9 ~\rm{dB}$}
	\end{minipage}
	\begin{minipage}{0.15\linewidth}
	\centering \small{$20.4 ~\rm{dB}$}
	\end{minipage}
	\begin{minipage}{0.15\linewidth}
	\centering \small{$39.1 ~\rm{dB}$}
	\end{minipage}
	\begin{minipage}{0.15\linewidth}
	\centering \small{$29.8 ~\rm{dB}$}
	\end{minipage} 

\caption{Results from real data. Reprentative examples of subtracted frame recovery from compressed measurements. Here, we consider a block sparse model fixed, with $g = 4$ block size per group. From top to bottom, the number of measurements range from $\lceil 0.25 \cdot \dim \rceil $ to $\lceil 0.4 \cdot \dim \rceil $, for $\dim = 2^{14}$. One can observe that one obtains better recovery as the number of measurements increases. } {\label{fig:004}}
\end{figure*}
